# Supplementary material for: V-ICAL Bench: Evaluating Video In-Context Learning for Multimodal Agents in Interactive Environments
Source: arXiv:2609.15683 source file (2026-10-09)
Supplement: Supplementary file 1 [file appendix_d_complete_episodes.tex]

% Auto-generated from batch_results; do not hand-edit individual rows.
\paragraph{Coverage.}
Each table below reports every decision round for one model on the same \texttt{CliffWalking-v1} initial state (configuration \texttt{4}, run 0). The current and post-action states are shown together with the complete visible rationale and executed action; the caption reports the episode-level normalized game score. Kimi-K3 is not included because its main-table result and corresponding episode logs are still pending.

\begingroup
\scriptsize
\setlength{\tabcolsep}{2pt}
\renewcommand{\arraystretch}{1.05}
\arrayrulecolor{black!18}
\begin{longtable}{@{}c c p{8.0cm} c c@{}}
\caption{Complete same-start-state episode: Seed-2.1-Pro on CliffWalking-v1 (4; victory; 8 steps; score 100).}
\label{tab:appendix-d-cliff-seed21}\\
\toprule
$t$ & Current state & Visible model rationale & Action & Next state \\
\midrule
\endfirsthead
\multicolumn{5}{c}{\tablename\ \thetable\ (continued)}\\
\toprule
$t$ & Current state & Visible model rationale & Action & Next state \\
\midrule
\endhead
\midrule
\multicolumn{5}{r}{Continued on next page}\\
\endfoot
\bottomrule
\endlastfoot
1 & \vcltopframe{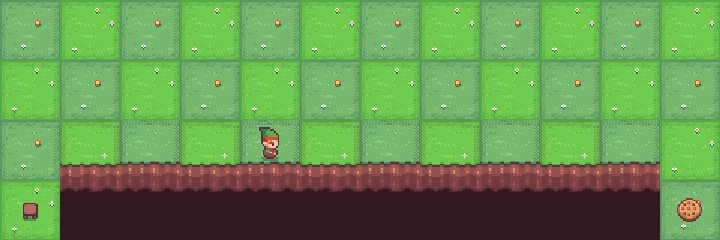} & \raggedright\ttfamily The goal (cookie) is at the bottom-right corner of the grid. The character is currently on the safe grass row directly above the cliff, to the left of the goal column. Moving down would cause the character to fall off the cliff immediately, moving left travels away from the goal, and moving up adds unnecessary extra steps. Moving right along this safe grass row toward the far-right column (above the goal) is the most direct, safe path to eventually reach the goal. & \texttt{Right} & \vcltopframe{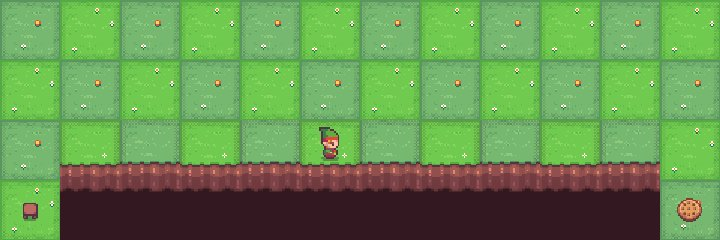} \\
\arrayrulecolor{black!12}\hline
2 & \vcltopframe{figures/content/appendix_d/episodes/cliff_seed21/frame_001.png} & \raggedright\ttfamily The character is still on the safe grass row above the cliff, and has not yet reached the far-right column above the goal. Moving down would result in falling off the cliff, moving left goes backward away from the goal, and moving up adds unnecessary steps. Continuing right along this safe row is the correct, direct path toward the goal. & \texttt{Right} & \vcltopframe{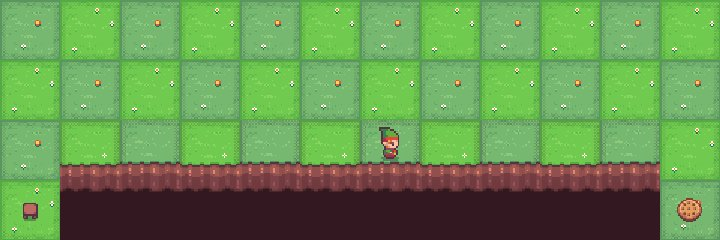} \\
\arrayrulecolor{black!12}\hline
3 & \vcltopframe{figures/content/appendix_d/episodes/cliff_seed21/frame_002.png} & \raggedright\ttfamily The character remains on the safe grass row directly above the cliff, and still has not reached the far-right column positioned over the goal. Moving down would cause a fatal fall off the cliff, moving left travels away from the goal, and moving up adds unnecessary detour steps. Continuing to move right along this safe row is the most efficient, safe progress toward the goal. & \texttt{Right} & \vcltopframe{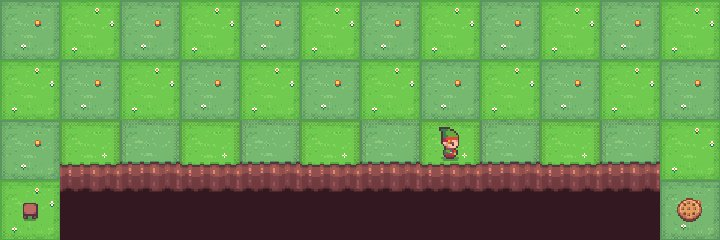} \\
\arrayrulecolor{black!12}\hline
4 & \vcltopframe{figures/content/appendix_d/episodes/cliff_seed21/frame_003.png} & \raggedright\ttfamily The character is still on the safe grass row above the cliff, and has not yet reached the far-right column that sits directly above the cookie goal. Moving down would lead to a fatal fall off the cliff, moving left reverses progress away from the goal, and moving up creates an unnecessary longer path. Continuing right along this safe row is the correct, efficient choice to progress toward the goal. & \texttt{Right} & \vcltopframe{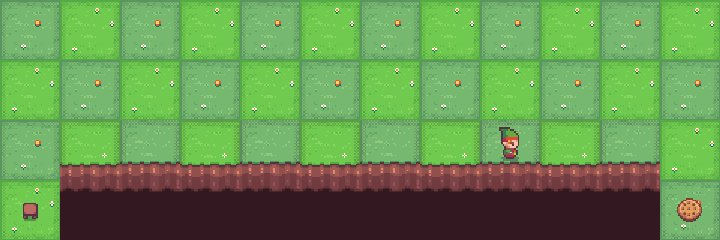} \\
\arrayrulecolor{black!12}\hline
5 & \vcltopframe{figures/content/appendix_d/episodes/cliff_seed21/frame_004.png} & \raggedright\ttfamily The character remains on the safe grass row above the cliff, and is still not positioned at the far-right column directly above the goal cookie. Moving down would cause a fatal cliff fall, moving left reverses hard-earned progress toward the goal, and moving up adds unnecessary detour steps. Continuing to move right along this safe row is the most efficient, safe path forward. & \texttt{Right} & \vcltopframe{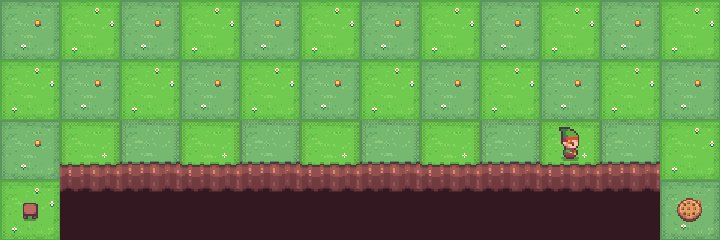} \\
\arrayrulecolor{black!12}\hline
6 & \vcltopframe{figures/content/appendix_d/episodes/cliff_seed21/frame_005.png} & \raggedright\ttfamily The character is still on the safe grass row above the cliff, and has not yet reached the far-right column that sits directly above the goal cookie. Moving down at this point would result in a fatal fall off the cliff, moving left travels backward away from the goal, and moving up creates an unnecessary longer path. Continuing right along this safe row is the correct, efficient progress toward the goal. & \texttt{Right} & \vcltopframe{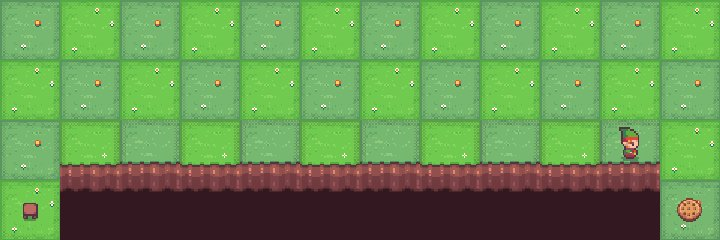} \\
\arrayrulecolor{black!12}\hline
7 & \vcltopframe{figures/content/appendix_d/episodes/cliff_seed21/frame_006.png} & \raggedright\ttfamily The character is one cell away from the far-right column that sits directly above the goal cookie. Moving down at this position would land on the cliff (fatal fall), moving left reverses progress, and moving up adds unnecessary steps. Moving right once more positions the character directly above the goal, setting up the final downward move to reach victory. & \texttt{Right} & \vcltopframe{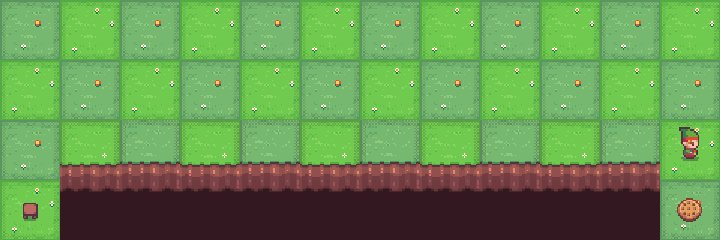} \\
\arrayrulecolor{black!12}\hline
8 & \vcltopframe{figures/content/appendix_d/episodes/cliff_seed21/frame_007.png} & \raggedright\ttfamily The character is now positioned directly above the goal cookie in the far-right column. Moving right is impossible (edge of the grid), moving left travels backward away from the goal, and moving up goes away from the goal. Moving down from this position lands directly on the goal cookie, which completes the game successfully. & \texttt{Down} & \vcltopframe{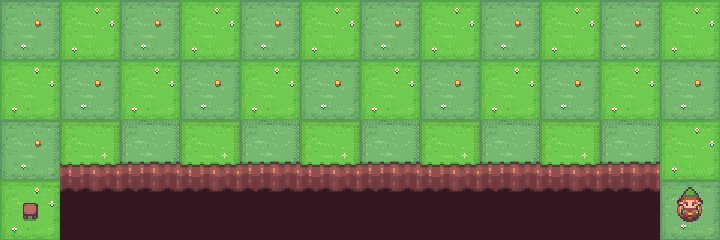} \\
\end{longtable}
\arrayrulecolor{black}
\endgroup

\begingroup
\scriptsize
\setlength{\tabcolsep}{2pt}
\renewcommand{\arraystretch}{1.05}
\arrayrulecolor{black!18}
\begin{longtable}{@{}c c p{8.0cm} c c@{}}
\caption{Complete same-start-state episode: Gemini-3.6-Flash on CliffWalking-v1 (4; victory; 8 steps; score 100).}
\label{tab:appendix-d-cliff-gemini36}\\
\toprule
$t$ & Current state & Visible model rationale & Action & Next state \\
\midrule
\endfirsthead
\multicolumn{5}{c}{\tablename\ \thetable\ (continued)}\\
\toprule
$t$ & Current state & Visible model rationale & Action & Next state \\
\midrule
\endhead
\midrule
\multicolumn{5}{r}{Continued on next page}\\
\endfoot
\bottomrule
\endlastfoot
1 & \vcltopframe{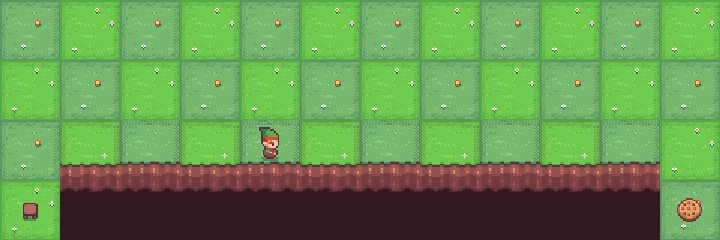} & \raggedright\ttfamily To reach the target cookie at the bottom-right corner safely and efficiently within the 16-step limit: - The character is currently at row 2, column 3 (just above the cliff edge). - Moving **Right** along row 2 allows the character to travel straight towards column 11 while remaining on safe grass, avoiding the cliff directly below at row 3. & \texttt{Right} & \vcltopframe{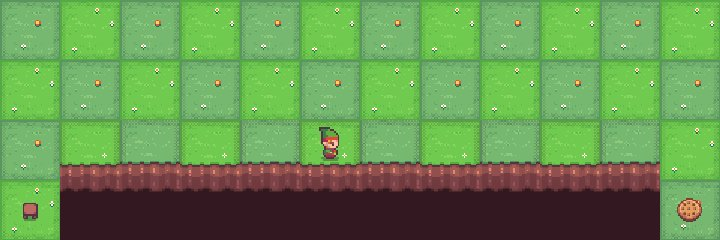} \\
\arrayrulecolor{black!12}\hline
2 & \vcltopframe{figures/content/appendix_d/episodes/cliff_gemini36/frame_001.png} & \raggedright\ttfamily Continuing to move right along row 2 towards column 11 to stay safely above the cliff. & \texttt{Right} & \vcltopframe{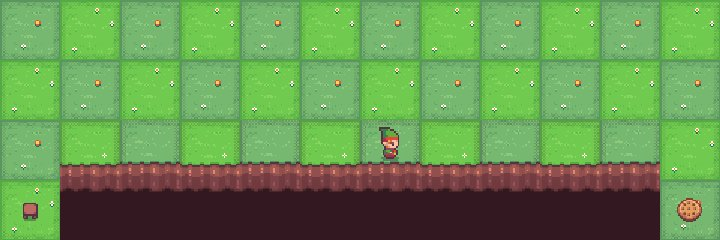} \\
\arrayrulecolor{black!12}\hline
3 & \vcltopframe{figures/content/appendix_d/episodes/cliff_gemini36/frame_002.png} & \raggedright\ttfamily Continuing to move right along row 2 towards column 11. & \texttt{Right} & \vcltopframe{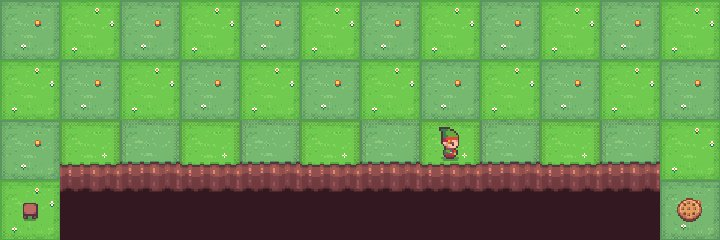} \\
\arrayrulecolor{black!12}\hline
4 & \vcltopframe{figures/content/appendix_d/episodes/cliff_gemini36/frame_003.png} & \raggedright\ttfamily Continuing to move right along row 2 towards the rightmost column above the goal tile. & \texttt{Right} & \vcltopframe{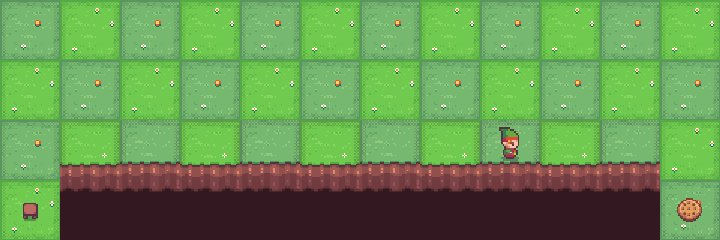} \\
\arrayrulecolor{black!12}\hline
5 & \vcltopframe{figures/content/appendix_d/episodes/cliff_gemini36/frame_004.png} & \raggedright\ttfamily Continuing right along row 2 toward the rightmost column above the cookie goal. & \texttt{Right} & \vcltopframe{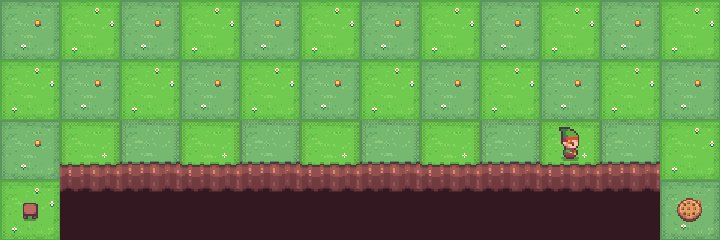} \\
\arrayrulecolor{black!12}\hline
6 & \vcltopframe{figures/content/appendix_d/episodes/cliff_gemini36/frame_005.png} & \raggedright\ttfamily Continuing to move right along row 2 to safely reach the rightmost column above the cookie goal, avoiding the cliff below. & \texttt{Right} & \vcltopframe{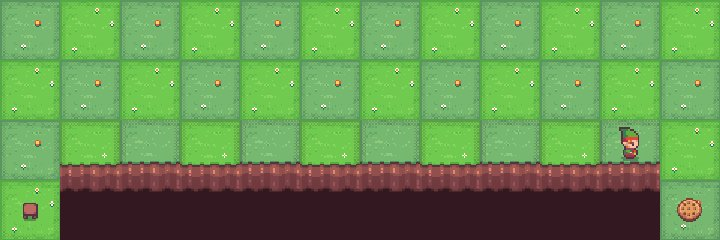} \\
\arrayrulecolor{black!12}\hline
7 & \vcltopframe{figures/content/appendix_d/episodes/cliff_gemini36/frame_006.png} & \raggedright\ttfamily Moving right into the rightmost column (column 11). Once in column 11, moving down will lead straight to the goal cookie. & \texttt{Right} & \vcltopframe{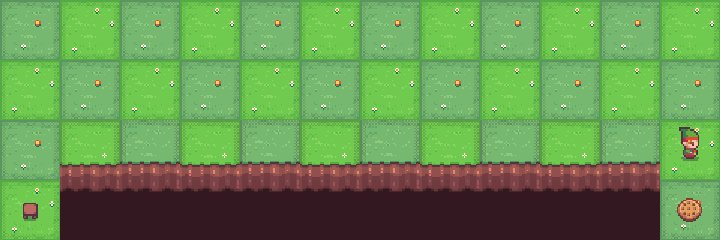} \\
\arrayrulecolor{black!12}\hline
8 & \vcltopframe{figures/content/appendix_d/episodes/cliff_gemini36/frame_007.png} & \raggedright\ttfamily We are now at the top of column 11, directly above the cookie goal. Moving Down will head towards the goal tile. & \texttt{Down} & \vcltopframe{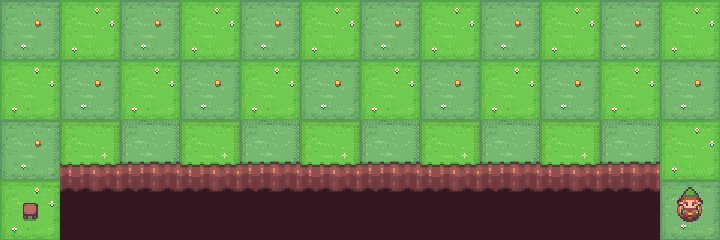} \\
\end{longtable}
\arrayrulecolor{black}
\endgroup

\begingroup
\scriptsize
\setlength{\tabcolsep}{2pt}
\renewcommand{\arraystretch}{1.05}
\arrayrulecolor{black!18}
\begin{longtable}{@{}c c p{8.0cm} c c@{}}
\caption{Complete same-start-state episode: Gemini-3.1-Pro on CliffWalking-v1 (4; victory; 8 steps; score 100).}
\label{tab:appendix-d-cliff-gemini31}\\
\toprule
$t$ & Current state & Visible model rationale & Action & Next state \\
\midrule
\endfirsthead
\multicolumn{5}{c}{\tablename\ \thetable\ (continued)}\\
\toprule
$t$ & Current state & Visible model rationale & Action & Next state \\
\midrule
\endhead
\midrule
\multicolumn{5}{r}{Continued on next page}\\
\endfoot
\bottomrule
\endlastfoot
1 & \vcltopframe{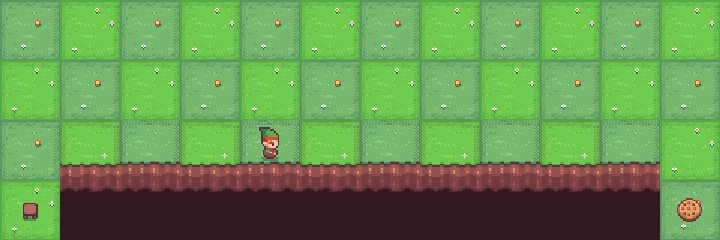} & \raggedright\ttfamily The character is currently on the row just above the cliff. To reach the goal at the bottom right without falling off the cliff, the character should continue moving to the right until it reaches the final column, where it can safely move down to the goal. Moving down right now would result in falling off the cliff and failing the game. & \texttt{Right} & \vcltopframe{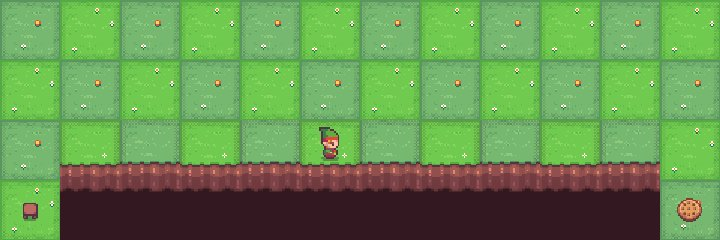} \\
\arrayrulecolor{black!12}\hline
2 & \vcltopframe{figures/content/appendix_d/episodes/cliff_gemini31/frame_001.png} & \raggedright\ttfamily The character needs to continue moving right to reach the safe column on the far right before moving down to the goal. Moving down here would lead to the cliff. & \texttt{Right} & \vcltopframe{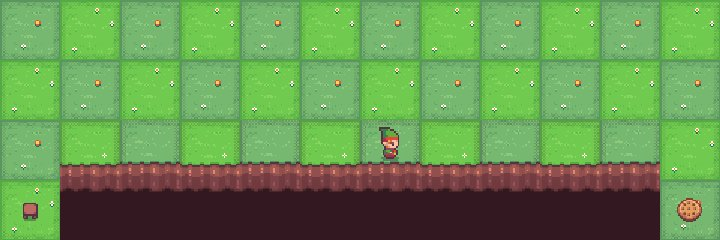} \\
\arrayrulecolor{black!12}\hline
3 & \vcltopframe{figures/content/appendix_d/episodes/cliff_gemini31/frame_002.png} & \raggedright\ttfamily The character must continue moving right along the safe row above the cliff to reach the rightmost column. Moving down would result in falling off the cliff. & \texttt{Right} & \vcltopframe{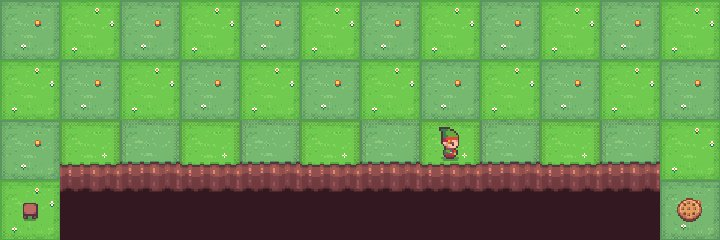} \\
\arrayrulecolor{black!12}\hline
4 & \vcltopframe{figures/content/appendix_d/episodes/cliff_gemini31/frame_003.png} & \raggedright\ttfamily The character is still on the row above the cliff. To safely reach the goal, it must continue moving right until it is in the same column as the goal. Moving down would cause the character to fall off the cliff. & \texttt{Right} & \vcltopframe{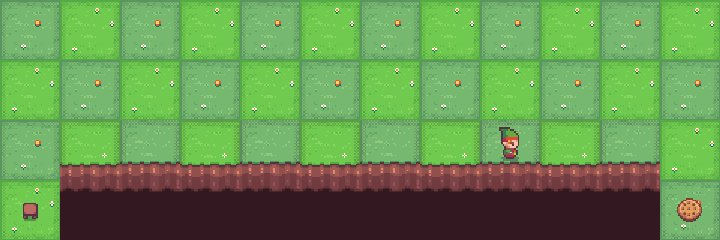} \\
\arrayrulecolor{black!12}\hline
5 & \vcltopframe{figures/content/appendix_d/episodes/cliff_gemini31/frame_004.png} & \raggedright\ttfamily The character needs to continue moving right along the safe path above the cliff. Moving down would result in falling off the cliff. & \texttt{Right} & \vcltopframe{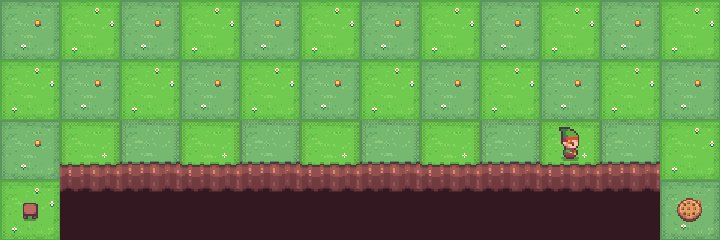} \\
\arrayrulecolor{black!12}\hline
6 & \vcltopframe{figures/content/appendix_d/episodes/cliff_gemini31/frame_005.png} & \raggedright\ttfamily The character must continue moving right to avoid the cliff directly below and reach the safe column on the far right. & \texttt{Right} & \vcltopframe{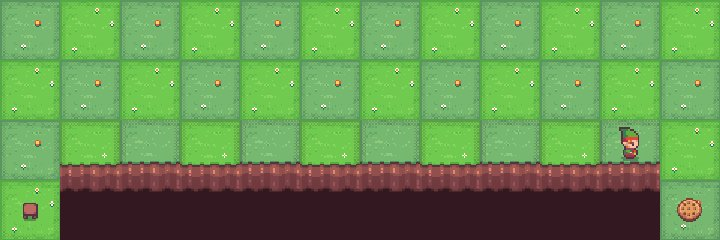} \\
\arrayrulecolor{black!12}\hline
7 & \vcltopframe{figures/content/appendix_d/episodes/cliff_gemini31/frame_006.png} & \raggedright\ttfamily The character is still above the cliff. It needs one more step to the right to reach the safe column where the goal is located. Moving down now would result in a failure. & \texttt{Right} & \vcltopframe{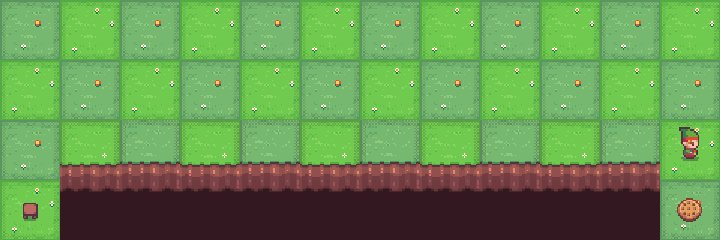} \\
\arrayrulecolor{black!12}\hline
8 & \vcltopframe{figures/content/appendix_d/episodes/cliff_gemini31/frame_007.png} & \raggedright\ttfamily The character has safely reached the rightmost column, which does not have a cliff. The goal is directly below, so moving down is the correct action to reach it. & \texttt{Down} & \vcltopframe{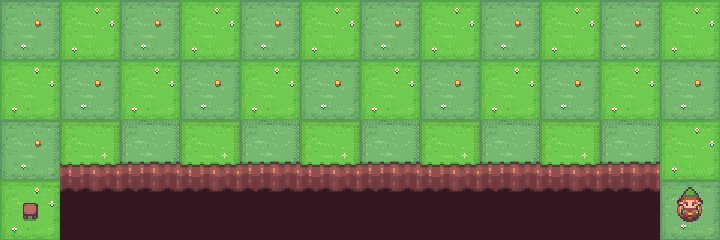} \\
\end{longtable}
\arrayrulecolor{black}
\endgroup

\begingroup
\scriptsize
\setlength{\tabcolsep}{2pt}
\renewcommand{\arraystretch}{1.05}
\arrayrulecolor{black!18}
\begin{longtable}{@{}c c p{8.0cm} c c@{}}
\caption{Complete same-start-state episode: GPT-5.6-sol on CliffWalking-v1 (4; victory; 10 steps; score 100).}
\label{tab:appendix-d-cliff-gpt56}\\
\toprule
$t$ & Current state & Visible model rationale & Action & Next state \\
\midrule
\endfirsthead
\multicolumn{5}{c}{\tablename\ \thetable\ (continued)}\\
\toprule
$t$ & Current state & Visible model rationale & Action & Next state \\
\midrule
\endhead
\midrule
\multicolumn{5}{r}{Continued on next page}\\
\endfoot
\bottomrule
\endlastfoot
1 & \vcltopframe{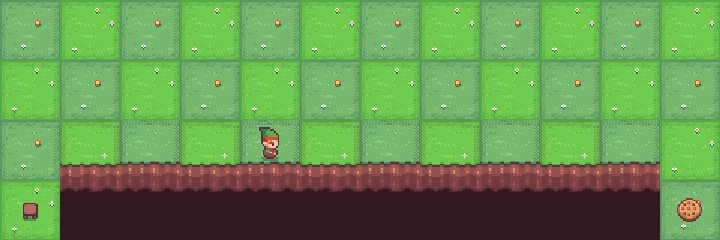} & \raggedright\ttfamily Move away from the cliff before heading right toward the goal. & \texttt{Up} & \vcltopframe{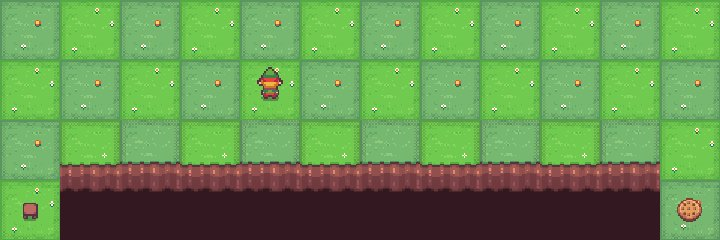} \\
\arrayrulecolor{black!12}\hline
2 & \vcltopframe{figures/content/appendix_d/episodes/cliff_gpt56/frame_001.png} & \raggedright\ttfamily Continue toward the goal while staying safely above the cliff. & \texttt{Right} & \vcltopframe{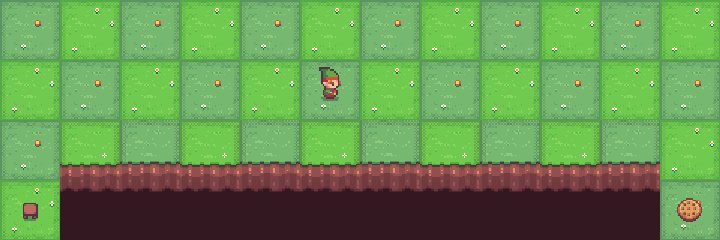} \\
\arrayrulecolor{black!12}\hline
3 & \vcltopframe{figures/content/appendix_d/episodes/cliff_gpt56/frame_002.png} & \raggedright\emph{No visible rationale.} & \texttt{Right} & \vcltopframe{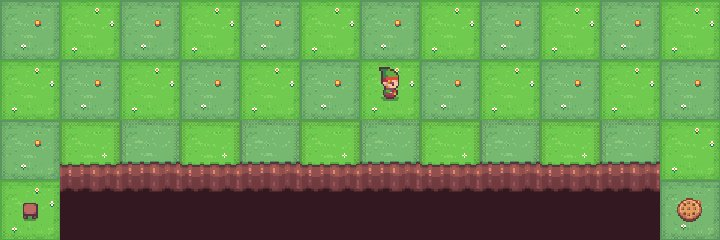} \\
\arrayrulecolor{black!12}\hline
4 & \vcltopframe{figures/content/appendix_d/episodes/cliff_gpt56/frame_003.png} & \raggedright\emph{No visible rationale.} & \texttt{Right} & \vcltopframe{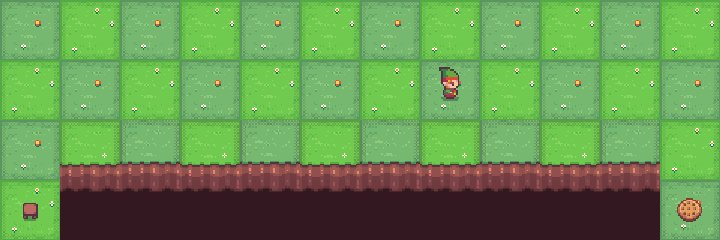} \\
\arrayrulecolor{black!12}\hline
5 & \vcltopframe{figures/content/appendix_d/episodes/cliff_gpt56/frame_004.png} & \raggedright\emph{No visible rationale.} & \texttt{Right} & \vcltopframe{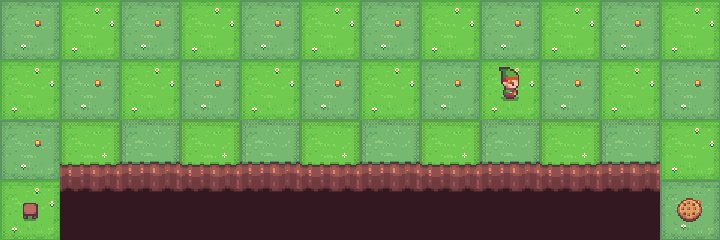} \\
\arrayrulecolor{black!12}\hline
6 & \vcltopframe{figures/content/appendix_d/episodes/cliff_gpt56/frame_005.png} & \raggedright\emph{No visible rationale.} & \texttt{Right} & \vcltopframe{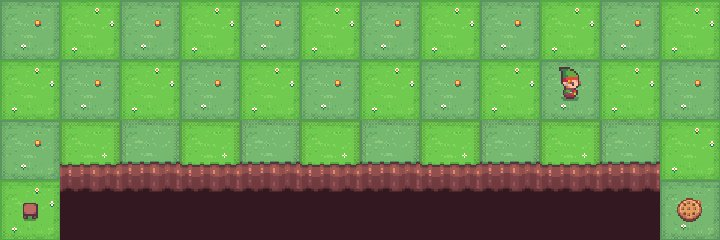} \\
\arrayrulecolor{black!12}\hline
7 & \vcltopframe{figures/content/appendix_d/episodes/cliff_gpt56/frame_006.png} & \raggedright\emph{No visible rationale.} & \texttt{Right} & \vcltopframe{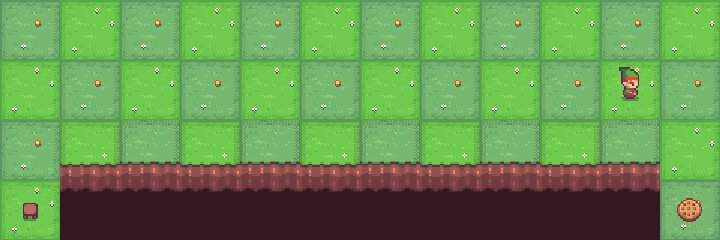} \\
\arrayrulecolor{black!12}\hline
8 & \vcltopframe{figures/content/appendix_d/episodes/cliff_gpt56/frame_007.png} & \raggedright\emph{No visible rationale.} & \texttt{Right} & \vcltopframe{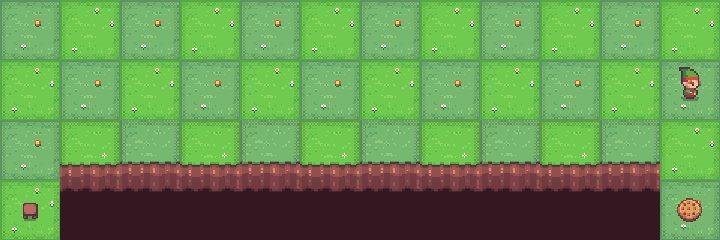} \\
\arrayrulecolor{black!12}\hline
9 & \vcltopframe{figures/content/appendix_d/episodes/cliff_gpt56/frame_008.png} & \raggedright\emph{No visible rationale.} & \texttt{Down} & \vcltopframe{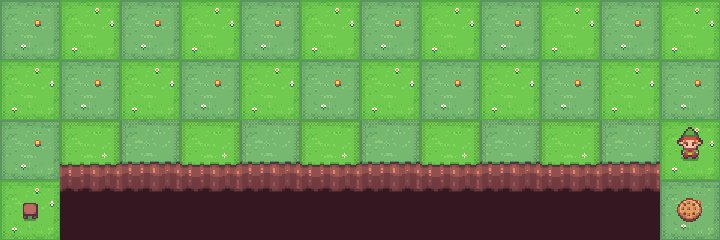} \\
\arrayrulecolor{black!12}\hline
10 & \vcltopframe{figures/content/appendix_d/episodes/cliff_gpt56/frame_009.png} & \raggedright\emph{No visible rationale.} & \texttt{Down} & \vcltopframe{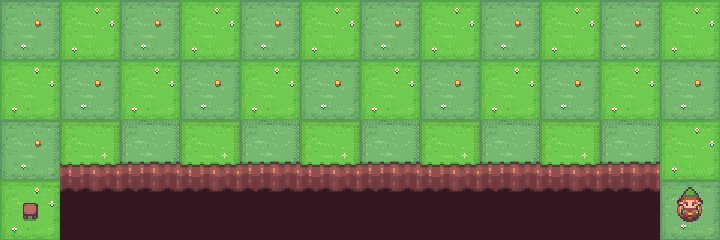} \\
\end{longtable}
\arrayrulecolor{black}
\endgroup

\begingroup
\scriptsize
\setlength{\tabcolsep}{2pt}
\renewcommand{\arraystretch}{1.05}
\arrayrulecolor{black!18}
\begin{longtable}{@{}c c p{8.0cm} c c@{}}
\caption{Complete same-start-state episode: Gemini-3-Flash on CliffWalking-v1 (4; gameover; 7 steps; score 77.14).}
\label{tab:appendix-d-cliff-gemini3}\\
\toprule
$t$ & Current state & Visible model rationale & Action & Next state \\
\midrule
\endfirsthead
\multicolumn{5}{c}{\tablename\ \thetable\ (continued)}\\
\toprule
$t$ & Current state & Visible model rationale & Action & Next state \\
\midrule
\endhead
\midrule
\multicolumn{5}{r}{Continued on next page}\\
\endfoot
\bottomrule
\endlastfoot
1 & \vcltopframe{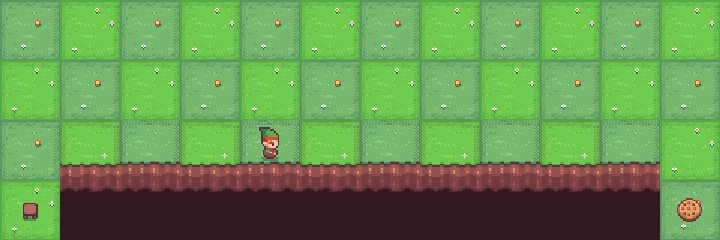} & \raggedright\ttfamily The character is currently at Row 2, Column 4. Moving Down would result in falling into the cliff at Row 3. To reach the goal at Row 3, Column 11 safely, the character must first move Right until they reach Column 11, then move Down. & \texttt{Right} & \vcltopframe{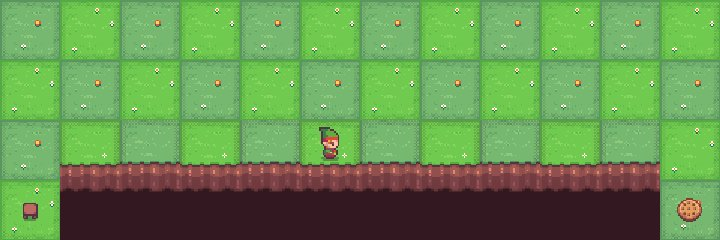} \\
\arrayrulecolor{black!12}\hline
2 & \vcltopframe{figures/content/appendix_d/episodes/cliff_gemini3/frame_001.png} & \raggedright\ttfamily The character is moving along the safe path above the cliff. I will continue moving Right towards the goal column. & \texttt{Right} & \vcltopframe{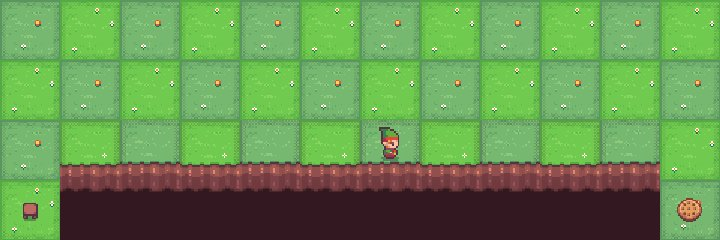} \\
\arrayrulecolor{black!12}\hline
3 & \vcltopframe{figures/content/appendix_d/episodes/cliff_gemini3/frame_002.png} & \raggedright\ttfamily The character is currently at Row 2, Column 6. To reach the goal at Row 3, Column 11 safely without falling into the cliff, I will continue moving Right along the safe path in Row 2 until I reach the final column. & \texttt{Right} & \vcltopframe{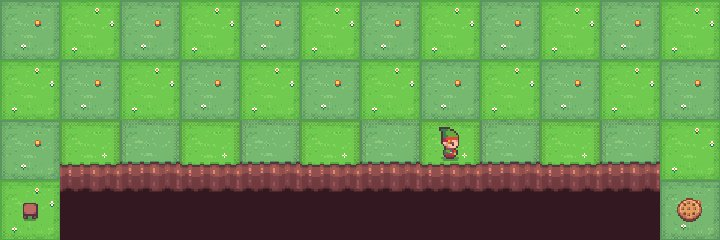} \\
\arrayrulecolor{black!12}\hline
4 & \vcltopframe{figures/content/appendix_d/episodes/cliff_gemini3/frame_003.png} & \raggedright\ttfamily The character is moving along the safe grass path in Row 2 to avoid the cliff in Row 3. I will continue moving Right towards the goal column. & \texttt{Right} & \vcltopframe{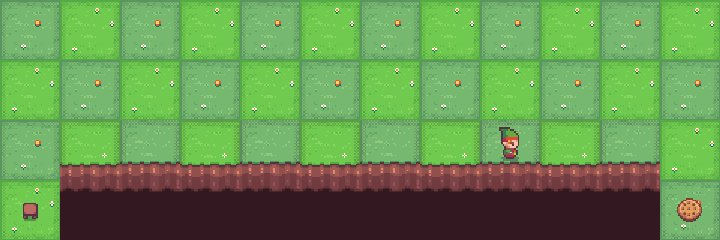} \\
\arrayrulecolor{black!12}\hline
5 & \vcltopframe{figures/content/appendix_d/episodes/cliff_gemini3/frame_004.png} & \raggedright\ttfamily The character is moving along the safe path in Row 2. I will continue moving Right to reach the final column before moving Down to the goal. & \texttt{Right} & \vcltopframe{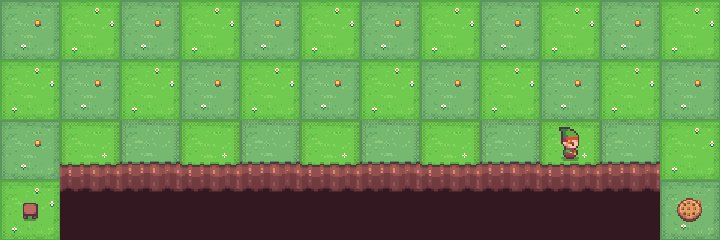} \\
\arrayrulecolor{black!12}\hline
6 & \vcltopframe{figures/content/appendix_d/episodes/cliff_gemini3/frame_005.png} & \raggedright\ttfamily The character is currently at Row 2, Column 10. To reach the goal at Row 3, Column 11 without falling into the cliff (which occupies Row 3, Columns 1-10), the character should move Right to Column 11 first, then move Down. & \texttt{Right} & \vcltopframe{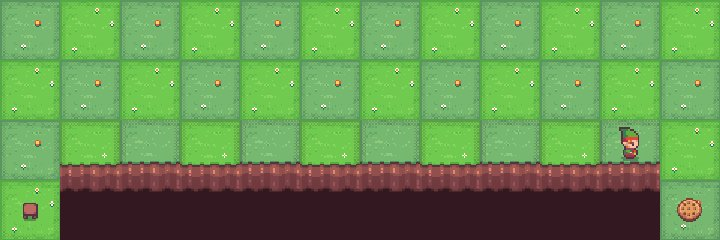} \\
\arrayrulecolor{black!12}\hline
7 & \vcltopframe{figures/content/appendix_d/episodes/cliff_gemini3/frame_006.png} & \raggedright\ttfamily The character is now in the final column (Column 11), directly above the goal. Moving Down will lead to the goal (the cookie) and complete the game safely, avoiding the cliff. & \texttt{Down} & \vcltopframe{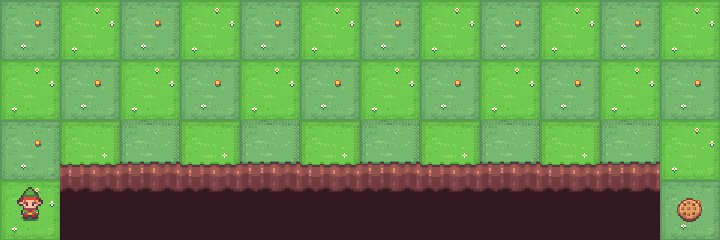} \\
\end{longtable}
\arrayrulecolor{black}
\endgroup

\begingroup
\scriptsize
\setlength{\tabcolsep}{2pt}
\renewcommand{\arraystretch}{1.05}
\arrayrulecolor{black!18}
\begin{longtable}{@{}c c p{8.0cm} c c@{}}
\caption{Complete same-start-state episode: Seed-2.0-Lite on CliffWalking-v1 (4; victory; 8 steps; score 100).}
\label{tab:appendix-d-cliff-seed20}\\
\toprule
$t$ & Current state & Visible model rationale & Action & Next state \\
\midrule
\endfirsthead
\multicolumn{5}{c}{\tablename\ \thetable\ (continued)}\\
\toprule
$t$ & Current state & Visible model rationale & Action & Next state \\
\midrule
\endhead
\midrule
\multicolumn{5}{r}{Continued on next page}\\
\endfoot
\bottomrule
\endlastfoot
1 & \vcltopframe{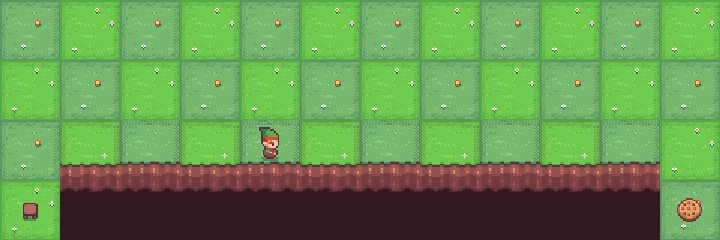} & \raggedright\ttfamily The elf is currently on the safe grass row directly above the long continuous cliff edge. Moving right keeps the character on valid non-cliff ground, progressing towards the far right side of the grid where the target cookie is located, and avoids accidentally falling off the cliff immediately. & \texttt{Right} & \vcltopframe{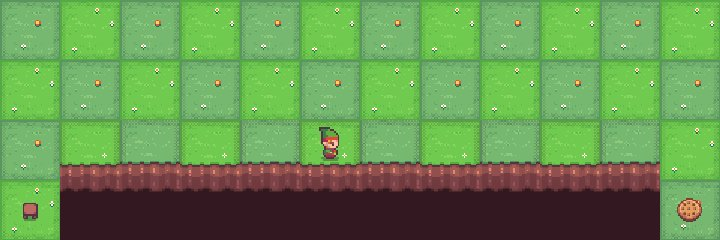} \\
\arrayrulecolor{black!12}\hline
2 & \vcltopframe{figures/content/appendix_d/episodes/cliff_seed20/frame_001.png} & \raggedright\ttfamily Continuing to move right along this safe grass row keeps progressing the elf closer to the far-right side of the grid where the target cookie is placed, and we avoid stepping onto the cliff directly below us for now. & \texttt{Right} & \vcltopframe{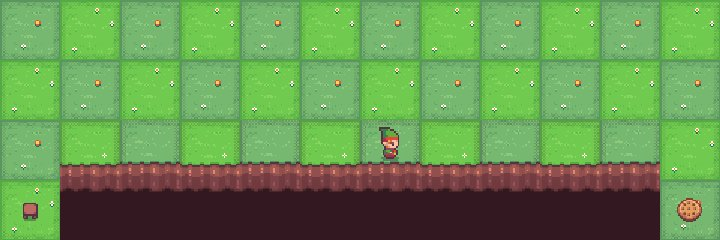} \\
\arrayrulecolor{black!12}\hline
3 & \vcltopframe{figures/content/appendix_d/episodes/cliff_seed20/frame_002.png} & \raggedright\ttfamily We are still on the safe grass row above the long cliff, moving right continues to close the distance to the far-right goal tile that holds the cookie, with no risk of falling off the cliff at this position. & \texttt{Right} & \vcltopframe{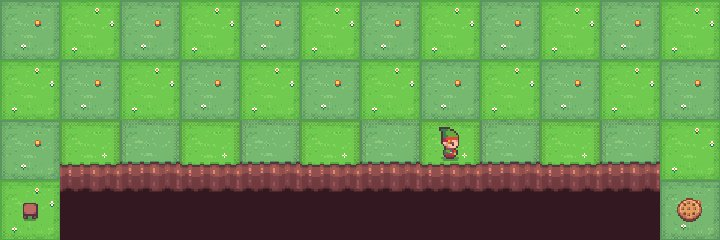} \\
\arrayrulecolor{black!12}\hline
4 & \vcltopframe{figures/content/appendix_d/episodes/cliff_seed20/frame_003.png} & \raggedright\ttfamily The elf remains on the safe grass row directly above the cliff edge, continuing to move right brings us closer to the far-rightmost cell on this row that is above the target cookie, avoiding any chance of falling off the cliff for now. & \texttt{Right} & \vcltopframe{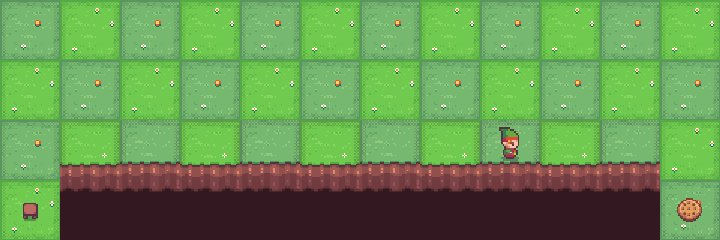} \\
\arrayrulecolor{black!12}\hline
5 & \vcltopframe{figures/content/appendix_d/episodes/cliff_seed20/frame_004.png} & \raggedright\ttfamily We are still on the valid safe grass tile, moving right further reduces the remaining distance to the far-right end of this row, where we will be able to safely move down to reach the cookie target without falling off the cliff. & \texttt{Right} & \vcltopframe{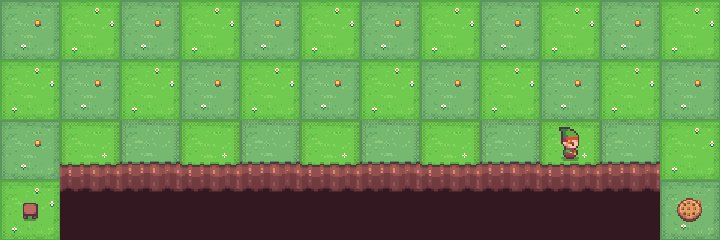} \\
\arrayrulecolor{black!12}\hline
6 & \vcltopframe{figures/content/appendix_d/episodes/cliff_seed20/frame_005.png} & \raggedright\ttfamily Continuing to move right along this safe grass path, we are now very close to the far-rightmost cell on this row that sits directly above the cookie's target position, so this step keeps us on track without any cliff fall danger. & \texttt{Right} & \vcltopframe{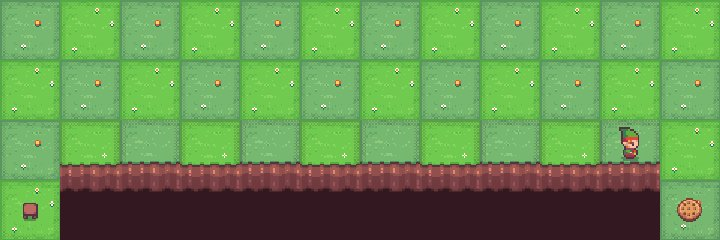} \\
\arrayrulecolor{black!12}\hline
7 & \vcltopframe{figures/content/appendix_d/episodes/cliff_seed20/frame_006.png} & \raggedright\ttfamily This move will take the elf to the far-rightmost safe cell on this row, the only position in this upper row where moving down will not cause us to fall into the cliff, and lands us directly above the cookie target. & \texttt{Right} & \vcltopframe{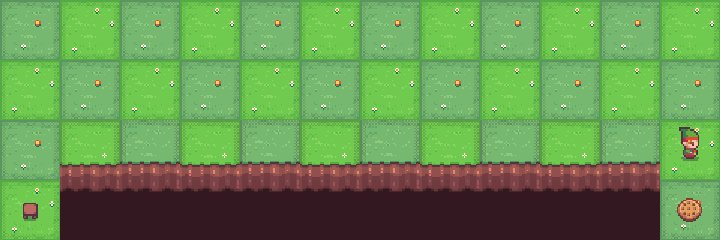} \\
\arrayrulecolor{black!12}\hline
8 & \vcltopframe{figures/content/appendix_d/episodes/cliff_seed20/frame_007.png} & \raggedright\ttfamily The elf is now positioned directly above the target cookie on the far right edge of the grid. Moving down will land us exactly on the goal tile, collecting the cookie and completing the game without falling off the cliff. & \texttt{Down} & \vcltopframe{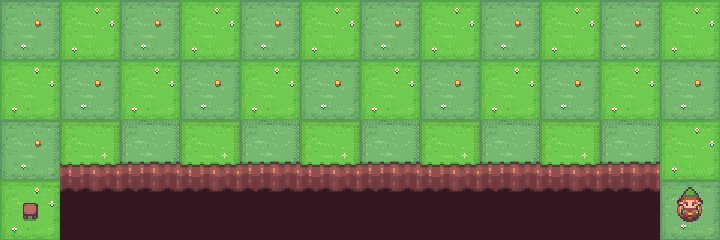} \\
\end{longtable}
\arrayrulecolor{black}
\endgroup

\begingroup
\scriptsize
\setlength{\tabcolsep}{2pt}
\renewcommand{\arraystretch}{1.05}
\arrayrulecolor{black!18}
\begin{longtable}{@{}c c p{8.0cm} c c@{}}
\caption{Complete same-start-state episode: Qwen3.5-397B-A17B on CliffWalking-v1 (4; victory; 8 steps; score 100).}
\label{tab:appendix-d-cliff-qwen35397}\\
\toprule
$t$ & Current state & Visible model rationale & Action & Next state \\
\midrule
\endfirsthead
\multicolumn{5}{c}{\tablename\ \thetable\ (continued)}\\
\toprule
$t$ & Current state & Visible model rationale & Action & Next state \\
\midrule
\endhead
\midrule
\multicolumn{5}{r}{Continued on next page}\\
\endfoot
\bottomrule
\endlastfoot
1 & \vcltopframe{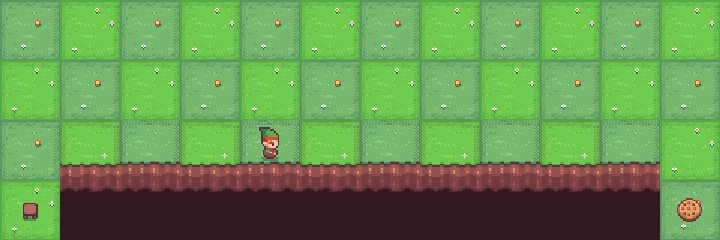} & \raggedright\ttfamily The character is currently on the row immediately above the cliff (Row 2). The goal is at the bottom-right corner. To reach the goal safely, the character needs to move to the rightmost column and then move down. Moving Right progresses towards the goal column while staying on safe ground. Moving Down would result in falling off the cliff. Moving Left moves away from the goal. Moving Up is safe but less direct. Therefore, Right is the best action. & \texttt{Right} & \vcltopframe{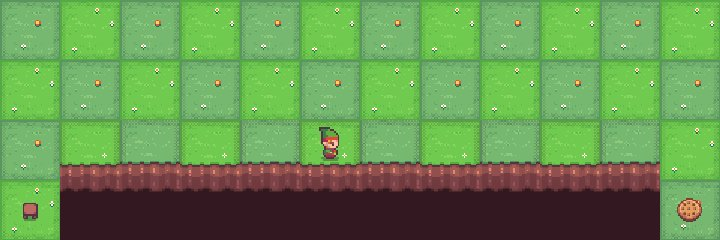} \\
\arrayrulecolor{black!12}\hline
2 & \vcltopframe{figures/content/appendix_d/episodes/cliff_qwen35397/frame_001.png} & \raggedright\ttfamily The character is currently on the bottom row of safe grass (Row 2), directly above the cliff. The goal is to the far right. Moving Right progresses towards the goal column while staying on safe ground. Moving Down would result in falling into the cliff. Moving Left moves away from the goal. Moving Up is safe but unnecessary as the current row allows direct access to the goal column. & \texttt{Right} & \vcltopframe{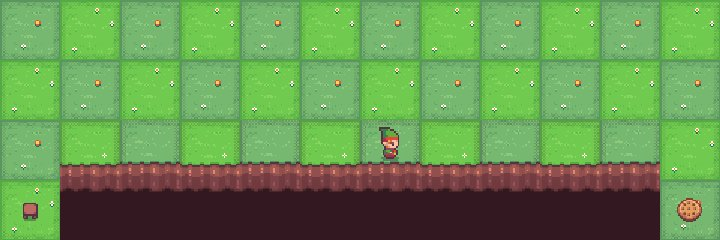} \\
\arrayrulecolor{black!12}\hline
3 & \vcltopframe{figures/content/appendix_d/episodes/cliff_qwen35397/frame_002.png} & \raggedright\ttfamily The character is currently on the second row from the bottom (Row 2), which is safe ground. The row below (Row 3) contains the cliff, except for the start and goal positions. Moving Down now would cause the character to fall off the cliff. To reach the goal at the bottom-right safely, the character must continue moving Right along the current row until reaching the far right column, and then move Down. Therefore, moving Right is the correct action. & \texttt{Right} & \vcltopframe{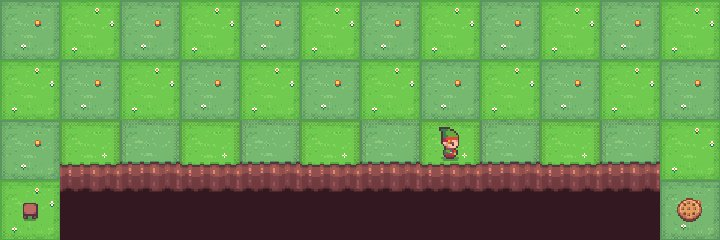} \\
\arrayrulecolor{black!12}\hline
4 & \vcltopframe{figures/content/appendix_d/episodes/cliff_qwen35397/frame_003.png} & \raggedright\ttfamily The character is currently on the third row from the top (Row 2), which is safe ground. The row below (Row 3) contains the "cliff" (the brown strip) in the middle columns, with the Start on the far left and Goal on the far right. Moving Down from the current position would result in falling into the cliff. To reach the goal safely, the character must continue moving Right along the current row until reaching the far right column, and then move Down to the goal. Therefore, moving Right is the correct action. & \texttt{Right} & \vcltopframe{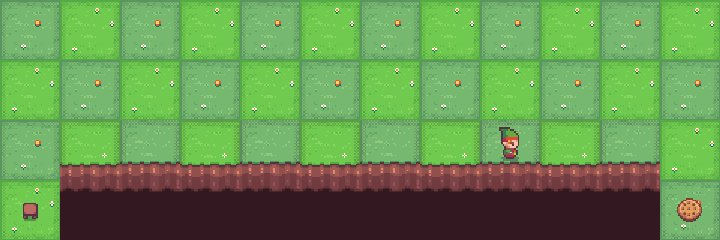} \\
\arrayrulecolor{black!12}\hline
5 & \vcltopframe{figures/content/appendix_d/episodes/cliff_qwen35397/frame_004.png} & \raggedright\ttfamily The character is currently on the row of safe grass directly above the cliff. Moving Down would cause the character to fall into the cliff and fail the game. To reach the goal (the cookie) at the bottom-right safely, the character must continue moving Right along this safe row until reaching the far right column, and only then move Down. Therefore, moving Right is the correct and safe action. & \texttt{Right} & \vcltopframe{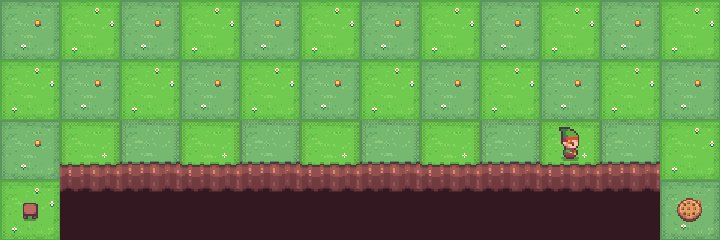} \\
\arrayrulecolor{black!12}\hline
6 & \vcltopframe{figures/content/appendix_d/episodes/cliff_qwen35397/frame_005.png} & \raggedright\ttfamily The character is currently on the safe row immediately above the cliff (Row 2). The goal is located at the bottom-right corner (Row 3, Column 11). The cliff occupies the bottom row from Column 1 to Column 10. Moving Down from the current position (approximately Column 9) would land the character on the cliff, resulting in failure. To reach the goal safely, the character must continue moving Right along the current row until reaching the column directly above the goal (Column 11), and then move Down. Therefore, moving Right is the correct action. & \texttt{Right} & \vcltopframe{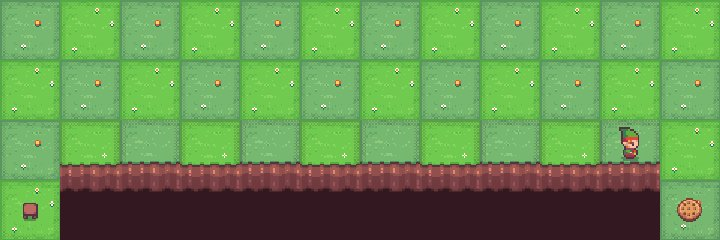} \\
\arrayrulecolor{black!12}\hline
7 & \vcltopframe{figures/content/appendix_d/episodes/cliff_qwen35397/frame_006.png} & \raggedright\ttfamily The character is currently on the bottom row of safe grass (Row 2), in the column immediately to the left of the goal column. Moving Down from this position would land the character on the cliff, resulting in failure. To reach the goal safely, the character must move Right into the far-right column (which is safe all the way down to the goal), and then move Down. Therefore, moving Right is the correct action. & \texttt{Right} & \vcltopframe{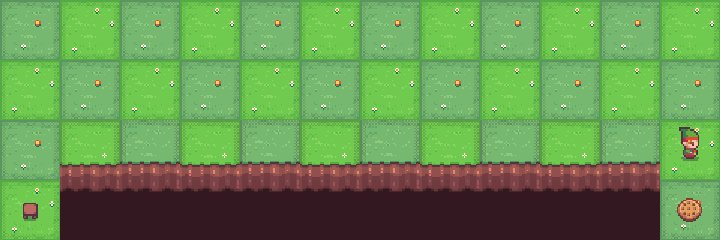} \\
\arrayrulecolor{black!12}\hline
8 & \vcltopframe{figures/content/appendix_d/episodes/cliff_qwen35397/frame_007.png} & \raggedright\ttfamily The character is currently in the far-right column, on the row directly above the bottom row. The goal (cookie) is located in the bottom-right corner. Since the far-right column is safe (unlike the middle columns which have the cliff), moving Down will place the character directly onto the goal, resulting in a victory. & \texttt{Down} & \vcltopframe{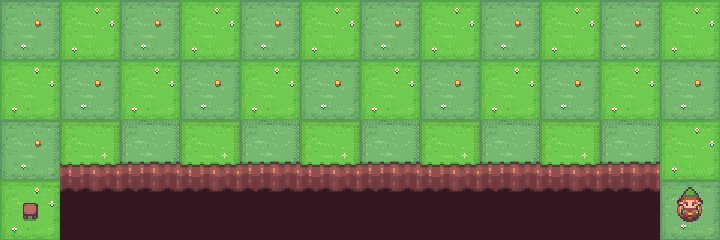} \\
\end{longtable}
\arrayrulecolor{black}
\endgroup

\begingroup
\scriptsize
\setlength{\tabcolsep}{2pt}
\renewcommand{\arraystretch}{1.05}
\arrayrulecolor{black!18}
\begin{longtable}{@{}c c p{8.0cm} c c@{}}
\caption{Complete same-start-state episode: gemma-4-31B-it on CliffWalking-v1 (4; victory; 10 steps; score 100).}
\label{tab:appendix-d-cliff-gemma4}\\
\toprule
$t$ & Current state & Visible model rationale & Action & Next state \\
\midrule
\endfirsthead
\multicolumn{5}{c}{\tablename\ \thetable\ (continued)}\\
\toprule
$t$ & Current state & Visible model rationale & Action & Next state \\
\midrule
\endhead
\midrule
\multicolumn{5}{r}{Continued on next page}\\
\endfoot
\bottomrule
\endlastfoot
1 & \vcltopframe{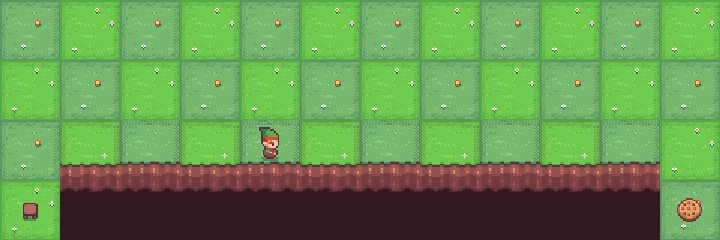} & \raggedright\ttfamily The player is currently standing on the edge of a cliff. Moving Down would lead to falling off the cliff and instant failure. Moving Right or Left is possible, but the goal (the cookie) is located on the far right. However, moving directly Right along the cliff edge is risky. Moving Up first creates a safe buffer between the player and the cliff, allowing for a safer path toward the objective. & \texttt{Up} & \vcltopframe{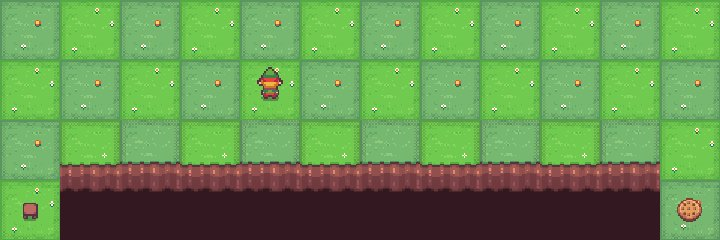} \\
\arrayrulecolor{black!12}\hline
2 & \vcltopframe{figures/content/appendix_d/episodes/cliff_gemma4/frame_001.png} & \raggedright\ttfamily Now that I have moved Up and am safely away from the cliff edge, I can move Right toward the goal (the cookie) without the risk of falling. & \texttt{Right} & \vcltopframe{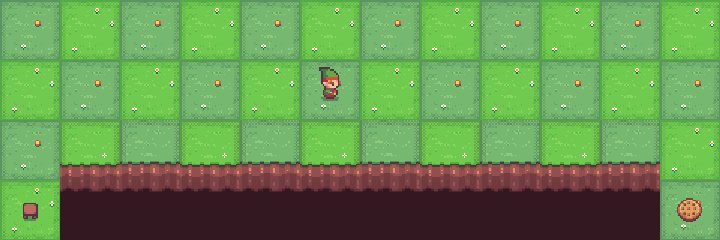} \\
\arrayrulecolor{black!12}\hline
3 & \vcltopframe{figures/content/appendix_d/episodes/cliff_gemma4/frame_002.png} & \raggedright\ttfamily Continuing to move Right towards the target goal (the cookie) while maintaining a safe distance from the cliff. & \texttt{Right} & \vcltopframe{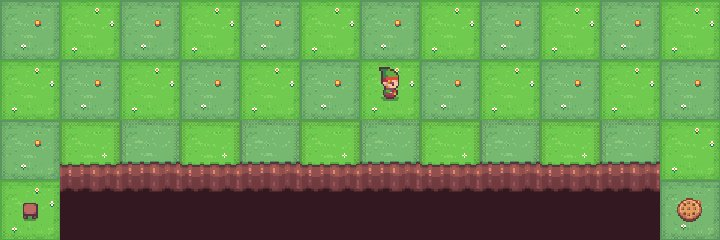} \\
\arrayrulecolor{black!12}\hline
4 & \vcltopframe{figures/content/appendix_d/episodes/cliff_gemma4/frame_003.png} & \raggedright\ttfamily Continuing the path to the right to reach the goal. & \texttt{Right} & \vcltopframe{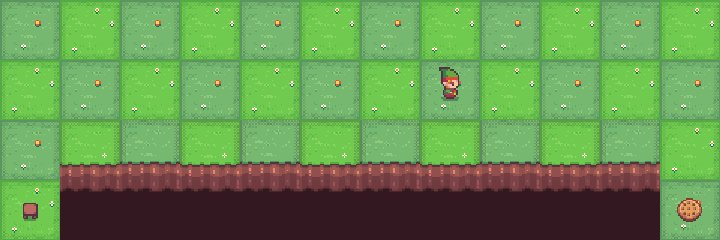} \\
\arrayrulecolor{black!12}\hline
5 & \vcltopframe{figures/content/appendix_d/episodes/cliff_gemma4/frame_004.png} & \raggedright\ttfamily Continuing to move right along the safe row toward the cookie. & \texttt{Right} & \vcltopframe{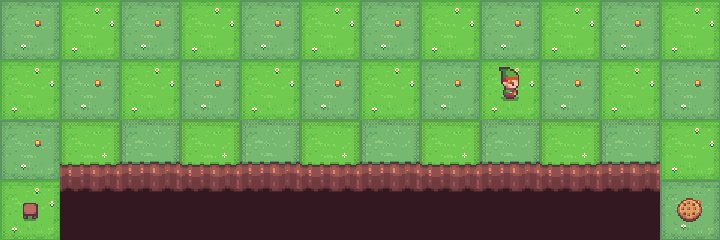} \\
\arrayrulecolor{black!12}\hline
6 & \vcltopframe{figures/content/appendix_d/episodes/cliff_gemma4/frame_005.png} & \raggedright\ttfamily Continuing the move Right to approach the target goal (the cookie). & \texttt{Right} & \vcltopframe{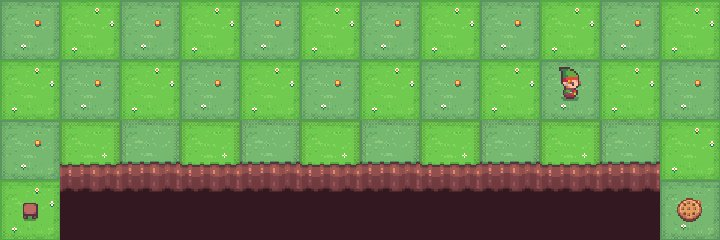} \\
\arrayrulecolor{black!12}\hline
7 & \vcltopframe{figures/content/appendix_d/episodes/cliff_gemma4/frame_006.png} & \raggedright\ttfamily I am continuing to move Right toward the goal (the cookie) while staying on the safe path. & \texttt{Right} & \vcltopframe{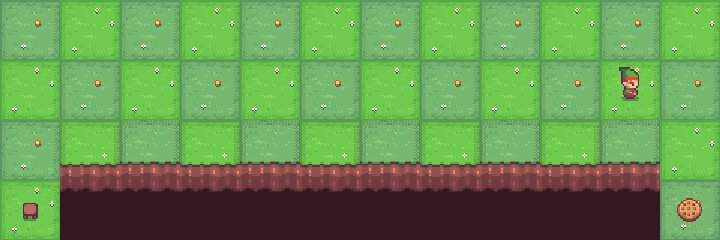} \\
\arrayrulecolor{black!12}\hline
8 & \vcltopframe{figures/content/appendix_d/episodes/cliff_gemma4/frame_007.png} & \raggedright\ttfamily Continuing to move right to reach the final column where the goal is located. & \texttt{Right} & \vcltopframe{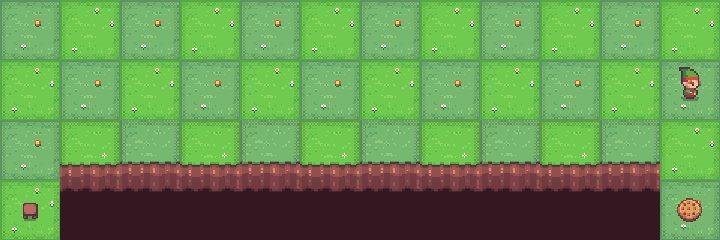} \\
\arrayrulecolor{black!12}\hline
9 & \vcltopframe{figures/content/appendix_d/episodes/cliff_gemma4/frame_008.png} & \raggedright\ttfamily I have reached the far right column. Now I need to move Down to reach the cookie goal located at the bottom of this column. & \texttt{Down} & \vcltopframe{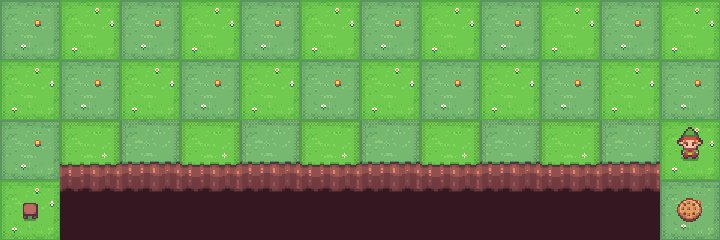} \\
\arrayrulecolor{black!12}\hline
10 & \vcltopframe{figures/content/appendix_d/episodes/cliff_gemma4/frame_009.png} & \raggedright\ttfamily I am in the final column and just one step away from the cookie goal. Moving Down will complete the objective. & \texttt{Down} & \vcltopframe{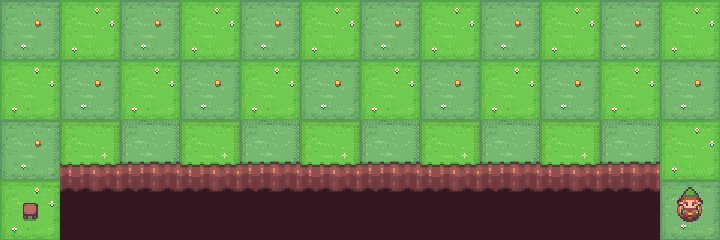} \\
\end{longtable}
\arrayrulecolor{black}
\endgroup

\begingroup
\scriptsize
\setlength{\tabcolsep}{2pt}
\renewcommand{\arraystretch}{1.05}
\arrayrulecolor{black!18}
\begin{longtable}{@{}c c p{8.0cm} c c@{}}
\caption{Complete same-start-state episode: MiMo-v2.5 on CliffWalking-v1 (4; victory; 13 steps; score 100).}
\label{tab:appendix-d-cliff-mimo25}\\
\toprule
$t$ & Current state & Visible model rationale & Action & Next state \\
\midrule
\endfirsthead
\multicolumn{5}{c}{\tablename\ \thetable\ (continued)}\\
\toprule
$t$ & Current state & Visible model rationale & Action & Next state \\
\midrule
\endhead
\midrule
\multicolumn{5}{r}{Continued on next page}\\
\endfoot
\bottomrule
\endlastfoot
1 & \vcltopframe{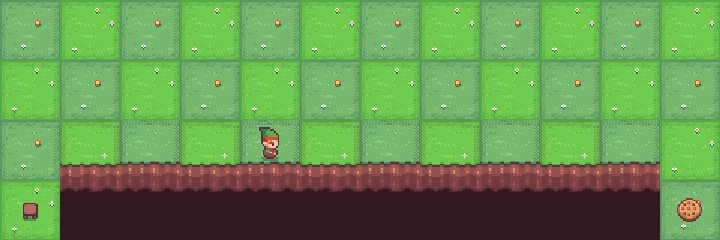} & \raggedright\ttfamily The goal of the game is to reach the pizza located in the bottom-right corner. The environment features a large cliff (the dark brown wall and black void) that blocks direct movement downwards from the middle of the map. In the current state, the character is positioned on the grass in the second row, near the center. Directly below the character is the cliff edge. Moving **Down** at this position would result in falling off the cliff and failing the game. The demonstration video showed that the safe path involves traversing horizontally along the top grassy area until reaching the far right side of the map, where there is a safe vertical path to the goal. Therefore, the correct action is to move **Right** to bypass the cliff and make progress toward the goal. & \texttt{Right} & \vcltopframe{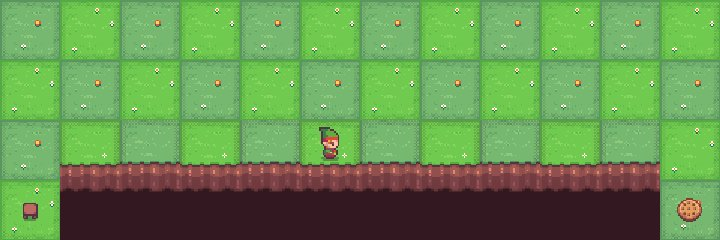} \\
\arrayrulecolor{black!12}\hline
2 & \vcltopframe{figures/content/appendix_d/episodes/cliff_mimo25/frame_001.png} & \raggedright\ttfamily The character needs to traverse to the far right side of the map to find a safe path down to the level where the pizza is located. Moving down from the current position would result in falling off the cliff, so the character must continue moving right. & \texttt{Right} & \vcltopframe{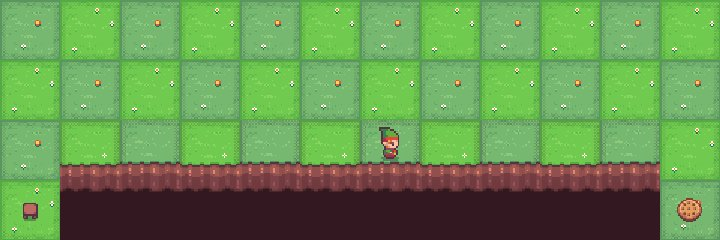} \\
\arrayrulecolor{black!12}\hline
3 & \vcltopframe{figures/content/appendix_d/episodes/cliff_mimo25/frame_002.png} & \raggedright\ttfamily The character is currently on the upper grassy level, above the cliff gap. To reach the goal (the pizza) located at the bottom right, the character must first traverse the map to the right side to find a safe path down. Moving down from the current position would result in falling off the cliff. Therefore, moving right is the correct step to progress toward the goal. & \texttt{Right} & \vcltopframe{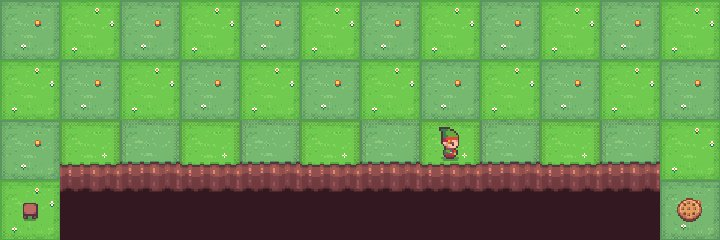} \\
\arrayrulecolor{black!12}\hline
4 & \vcltopframe{figures/content/appendix_d/episodes/cliff_mimo25/frame_003.png} & \raggedright\ttfamily The character needs to traverse to the far right of the map to find a safe path down to the level where the goal (the pizza) is located. Moving down from the current position would result in falling off the cliff. Therefore, continuing to move right is the correct action. & \texttt{Right} & \vcltopframe{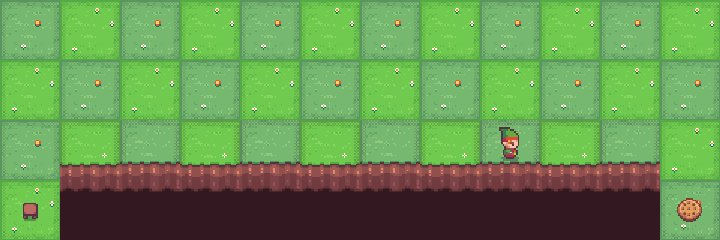} \\
\arrayrulecolor{black!12}\hline
5 & \vcltopframe{figures/content/appendix_d/episodes/cliff_mimo25/frame_004.png} & \raggedright\ttfamily The character is still on the upper grassy area above the cliff gap. To reach the goal (the pizza) at the bottom right, I need to continue moving right to reach the far side of the map where there is a safe path down. Moving down now would cause a fall, so right is the only safe progression. & \texttt{Right} & \vcltopframe{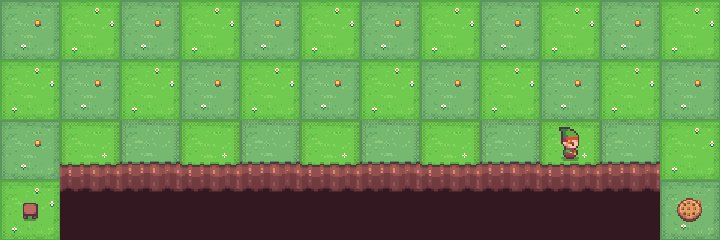} \\
\arrayrulecolor{black!12}\hline
6 & \vcltopframe{figures/content/appendix_d/episodes/cliff_mimo25/frame_005.png} & \raggedright\ttfamily The character is approaching the far right edge of the upper grassy area. I need to continue moving right to reach the safe descent path where I can then move down to reach the goal (the pizza) at the bottom right corner. Moving down now would still result in falling off the cliff. & \texttt{Right} & \vcltopframe{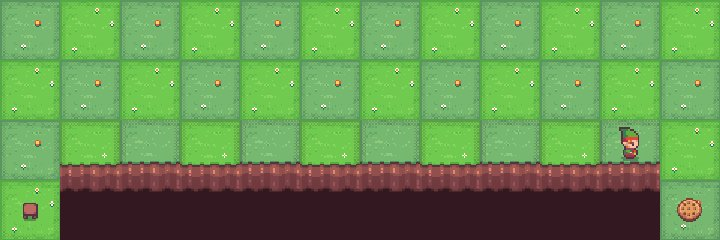} \\
\arrayrulecolor{black!12}\hline
7 & \vcltopframe{figures/content/appendix_d/episodes/cliff_mimo25/frame_006.png} & \raggedright\ttfamily The character is still on the upper grassy area and needs to continue moving right to reach the far right side of the map where there is a safe path down to the goal (the pizza). Moving down now would result in falling off the cliff. & \texttt{Right} & \vcltopframe{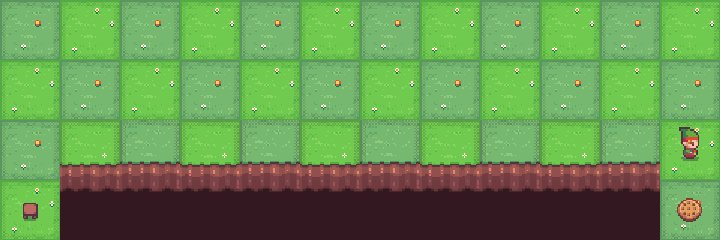} \\
\arrayrulecolor{black!12}\hline
8 & \vcltopframe{figures/content/appendix_d/episodes/cliff_mimo25/frame_007.png} & \raggedright\ttfamily The character needs to continue moving right along the upper grassy area to reach the far right side of the map. This is the only safe path to eventually descend to the level where the pizza goal is located. Moving down from the current position would cause a fall off the cliff. & \texttt{Right} & \vcltopframe{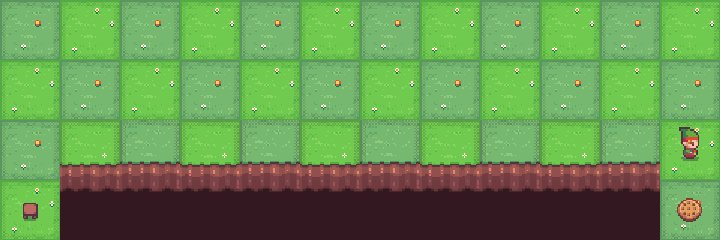} \\
\arrayrulecolor{black!12}\hline
9 & \vcltopframe{figures/content/appendix_d/episodes/cliff_mimo25/frame_008.png} & \raggedright\ttfamily The character needs to continue moving right along the upper grassy area to reach the far right side of the map. This is the only safe path to eventually descend to the level where the pizza goal is located. Looking at the current position, the character is getting closer to the right edge but isn't there yet. Moving down from the current position would cause a fall off the cliff, so continuing right is the correct action. & \texttt{Right} & \vcltopframe{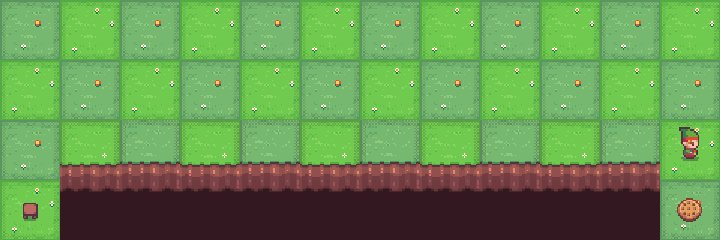} \\
\arrayrulecolor{black!12}\hline
10 & \vcltopframe{figures/content/appendix_d/episodes/cliff_mimo25/frame_009.png} & \raggedright\ttfamily The character is getting close to the right edge of the map but still needs to continue moving right. Once the character reaches the far right side, there should be a safe path down to reach the pizza goal. Moving down from the current position would still cause a fall off the cliff, so continuing right is the correct action. & \texttt{Right} & \vcltopframe{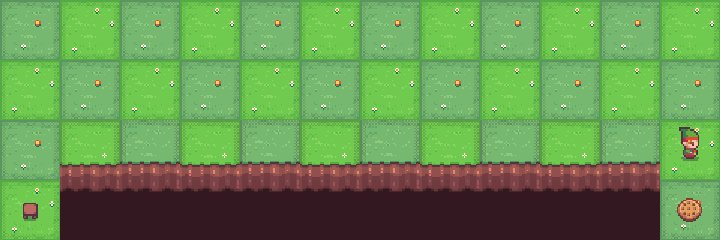} \\
\arrayrulecolor{black!12}\hline
11 & \vcltopframe{figures/content/appendix_d/episodes/cliff_mimo25/frame_010.png} & \raggedright\ttfamily The character is still on the upper grassy level and needs to continue moving right to reach the far right side of the map where there is a safe path down to reach the pizza goal. Moving down now would still result in falling off the cliff, so right is the correct action. & \texttt{Right} & \vcltopframe{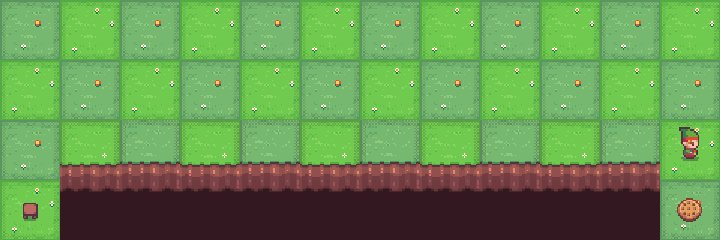} \\
\arrayrulecolor{black!12}\hline
12 & \vcltopframe{figures/content/appendix_d/episodes/cliff_mimo25/frame_011.png} & \raggedright\ttfamily The character is still on the upper grassy level above the cliff. To reach the pizza goal at the bottom right, I must continue moving right to reach the far right side of the map where there is a safe path down. Moving down from the current position would cause a fall off the cliff, so right is the correct action. & \texttt{Right} & \vcltopframe{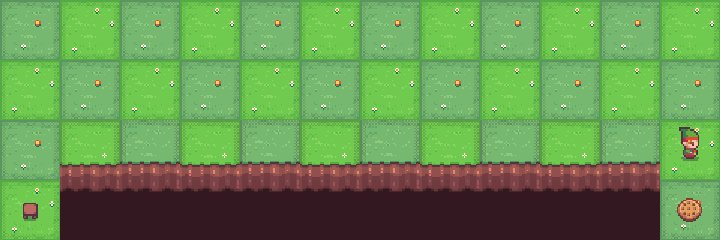} \\
\arrayrulecolor{black!12}\hline
13 & \vcltopframe{figures/content/appendix_d/episodes/cliff_mimo25/frame_012.png} & \raggedright\ttfamily The character has now reached the far right side of the map where the cliff edge ends. Looking at the current state, there is green grass below the character's current position, indicating a safe path down. Moving down now should lead toward the pizza goal at the bottom right corner. & \texttt{Down} & \vcltopframe{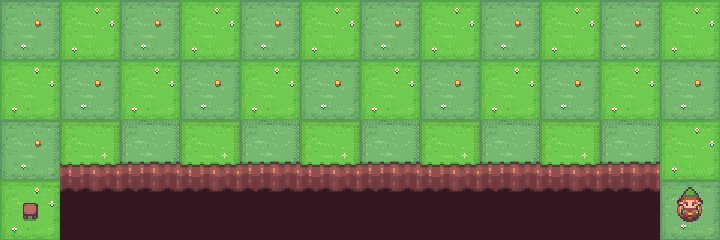} \\
\end{longtable}
\arrayrulecolor{black}
\endgroup

\begingroup
\scriptsize
\setlength{\tabcolsep}{2pt}
\renewcommand{\arraystretch}{1.05}
\arrayrulecolor{black!18}
\begin{longtable}{@{}c c p{8.0cm} c c@{}}
\caption{Complete same-start-state episode: Qwen2.5-72B on CliffWalking-v1 (4; gameover; 7 steps; score 77.14).}
\label{tab:appendix-d-cliff-qwen2572}\\
\toprule
$t$ & Current state & Visible model rationale & Action & Next state \\
\midrule
\endfirsthead
\multicolumn{5}{c}{\tablename\ \thetable\ (continued)}\\
\toprule
$t$ & Current state & Visible model rationale & Action & Next state \\
\midrule
\endhead
\midrule
\multicolumn{5}{r}{Continued on next page}\\
\endfoot
\bottomrule
\endlastfoot
1 & \vcltopframe{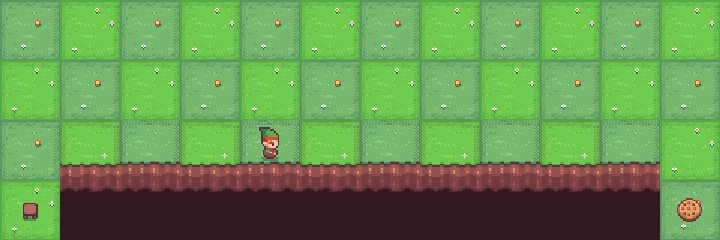} & \raggedright\ttfamily By moving right, I can continue progressing towards the goal while avoiding the cliff edge. This follows the strategy demonstrated in the example gameplay, where continuous movement to the right leads to victory. & \texttt{Right} & \vcltopframe{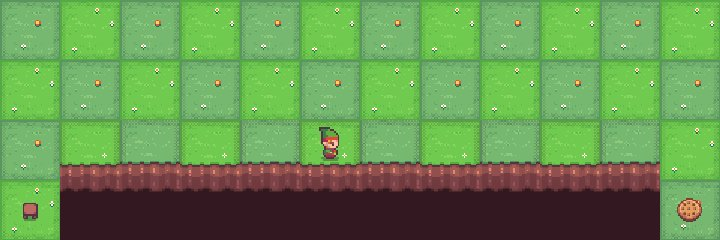} \\
\arrayrulecolor{black!12}\hline
2 & \vcltopframe{figures/content/appendix_d/episodes/cliff_qwen2572/frame_001.png} & \raggedright\ttfamily Continuing to move right will allow me to progress further towards the goal without risking falling off the cliff. This follows the successful path demonstrated in the example gameplay. & \texttt{Right} & \vcltopframe{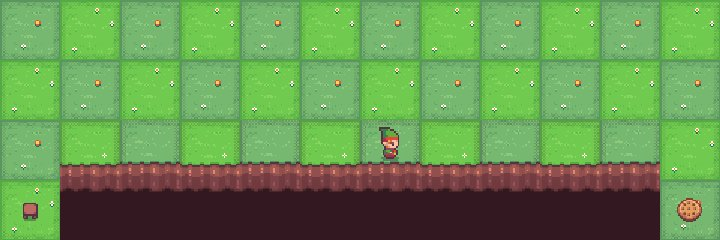} \\
\arrayrulecolor{black!12}\hline
3 & \vcltopframe{figures/content/appendix_d/episodes/cliff_qwen2572/frame_002.png} & \raggedright\ttfamily Moving right continues the path toward the goal while maintaining safety from the cliff. This aligns with the strategy observed in the example gameplay. & \texttt{Right} & \vcltopframe{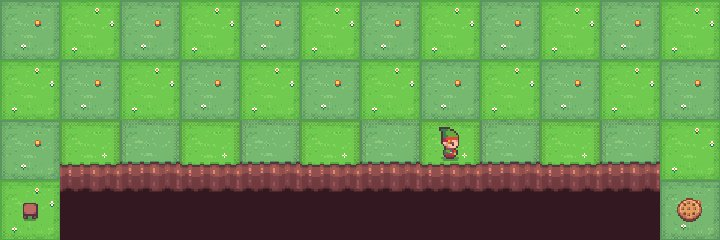} \\
\arrayrulecolor{black!12}\hline
4 & \vcltopframe{figures/content/appendix_d/episodes/cliff_qwen2572/frame_003.png} & \raggedright\ttfamily Continuing to move right will bring me closer to the goal while ensuring I avoid the cliff below. This aligns with the successful strategy from the example gameplay. & \texttt{Right} & \vcltopframe{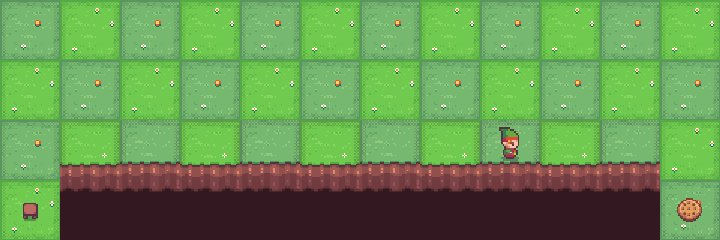} \\
\arrayrulecolor{black!12}\hline
5 & \vcltopframe{figures/content/appendix_d/episodes/cliff_qwen2572/frame_004.png} & \raggedright\ttfamily Moving right continues to advance towards the goal while staying away from the cliff, following the same successful strategy as seen in the example gameplay. & \texttt{Right} & \vcltopframe{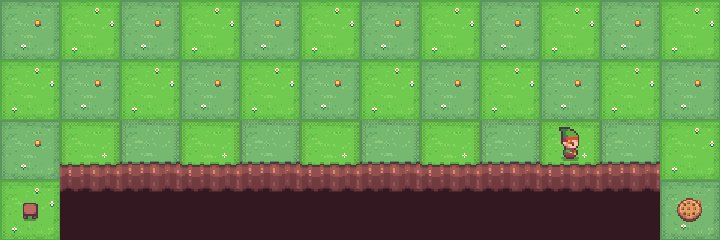} \\
\arrayrulecolor{black!12}\hline
6 & \vcltopframe{figures/content/appendix_d/episodes/cliff_qwen2572/frame_005.png} & \raggedright\ttfamily Continuing to move right will allow me to safely progress towards the goal while avoiding the cliff. This aligns with the successful strategy demonstrated in the gameplay example. & \texttt{Right} & \vcltopframe{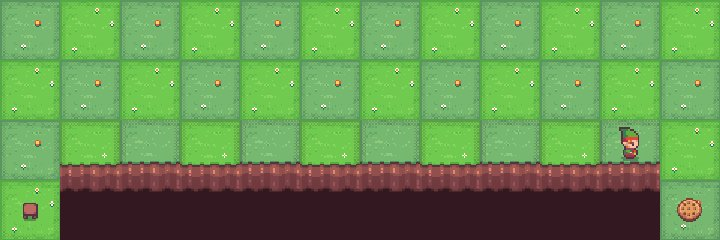} \\
\arrayrulecolor{black!12}\hline
7 & \vcltopframe{figures/content/appendix_d/episodes/cliff_qwen2572/frame_006.png} & \raggedright\ttfamily Since I've reached the column directly above the goal, moving down will allow me to reach it and secure victory. This aligns with the strategy displayed in the example gameplay. & \texttt{Down} & \vcltopframe{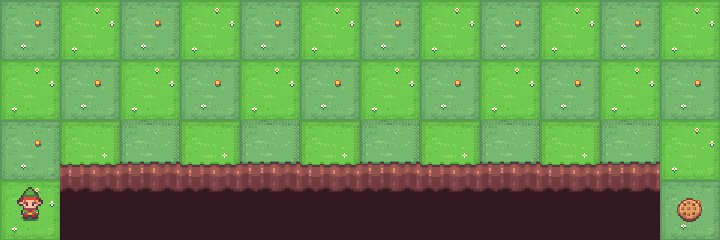} \\
\end{longtable}
\arrayrulecolor{black}
\endgroup

\begingroup
\scriptsize
\setlength{\tabcolsep}{2pt}
\renewcommand{\arraystretch}{1.05}
\arrayrulecolor{black!18}
\begin{longtable}{@{}c c p{8.0cm} c c@{}}
\caption{Complete same-start-state episode: MiMo-VL-7B on CliffWalking-v1 (4; victory; 11 steps; score 100).}
\label{tab:appendix-d-cliff-mimovl7}\\
\toprule
$t$ & Current state & Visible model rationale & Action & Next state \\
\midrule
\endfirsthead
\multicolumn{5}{c}{\tablename\ \thetable\ (continued)}\\
\toprule
$t$ & Current state & Visible model rationale & Action & Next state \\
\midrule
\endhead
\midrule
\multicolumn{5}{r}{Continued on next page}\\
\endfoot
\bottomrule
\endlastfoot
1 & \vcltopframe{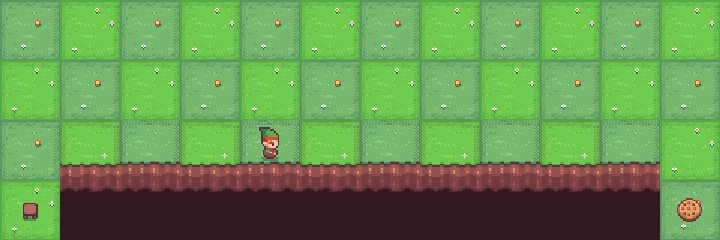} & \raggedright\ttfamily Got it, let's analyze the current initial state. The character is on a green platform, with a cliff below (the brownish-purple area). The goal is to reach the right side where there's a target (the brown circle) without falling. Let's think about the steps. The max steps are 16, so we need to move right towards the target. Wait, the current state: the character is in the middle of the green area. The cliff is the lower part. So moving right would keep them on the green platform. Let's check the example videos: in the first video, they moved right multiple times. So the best action is Right. Reasoning: The current state shows the character on a green platform above a cliff. To reach the target (brown circle on the right) without falling, moving right is the logical first step to stay on the safe platform and progress toward the goal. & \texttt{Right} & \vcltopframe{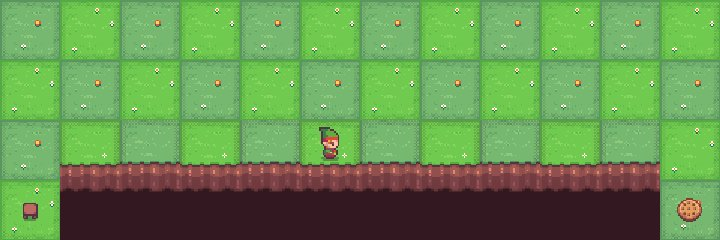} \\
\arrayrulecolor{black!12}\hline
2 & \vcltopframe{figures/content/appendix_d/episodes/cliff_mimovl7/frame_001.png} & \raggedright\ttfamily Got it, let's look at the current state. The character is on the green platform, right after moving right. The target is on the far right. So continuing to move right is the way to go. Need to stay on the green squares to avoid the cliff. So next action is Right. Reasoning: The character is still on the safe green platform, and moving right continues progress toward the target on the far right while avoiding the cliff below. & \texttt{Right} & \vcltopframe{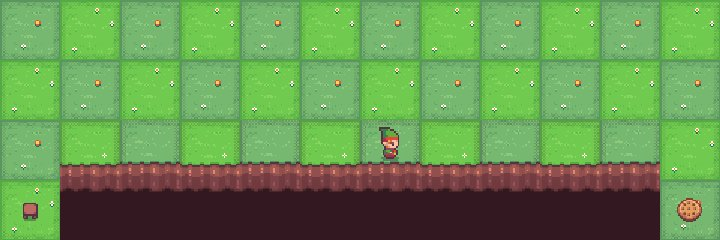} \\
\arrayrulecolor{black!12}\hline
3 & \vcltopframe{figures/content/appendix_d/episodes/cliff_mimovl7/frame_002.png} & \raggedright\ttfamily Got it, the character is moving right again. The target is still on the far right. So keep moving right to stay on the green platform and get closer. Need to avoid the cliff, so right is safe here. Reasoning: The character remains on the safe green platform, and moving right continues to advance toward the target while staying above the cliff. & \texttt{Right} & \vcltopframe{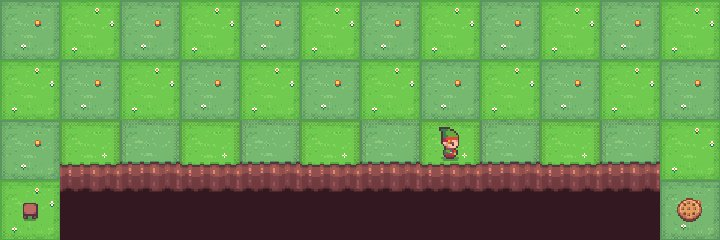} \\
\arrayrulecolor{black!12}\hline
4 & \vcltopframe{figures/content/appendix_d/episodes/cliff_mimovl7/frame_003.png} & \raggedright\ttfamily The character is still on the green platform. Moving right again is the best choice to keep progressing toward the target on the right. Staying on the green squares is key to not falling. Reasoning: The character is on the safe green platform, and moving right continues the progression toward the target on the far right while avoiding the cliff below. & \texttt{Right} & \vcltopframe{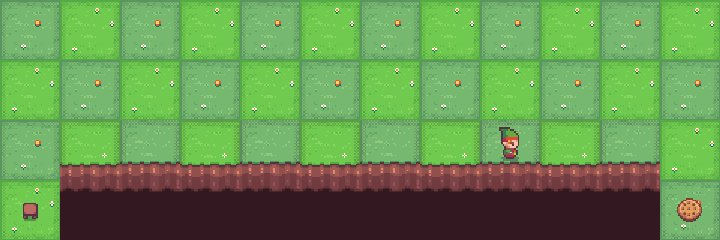} \\
\arrayrulecolor{black!12}\hline
5 & \vcltopframe{figures/content/appendix_d/episodes/cliff_mimovl7/frame_004.png} & \raggedright\ttfamily The pattern is moving right each time. The target is still on the right, so continuing right is logical. The character is on the green platform, so right keeps them safe. Reasoning: The character is on the safe green platform, and moving right is the optimal choice to continue advancing toward the target on the far right without falling into the cliff. & \texttt{Right} & \vcltopframe{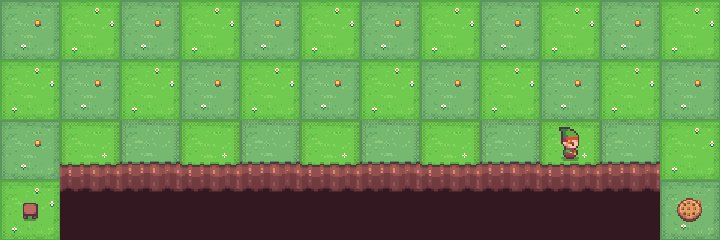} \\
\arrayrulecolor{black!12}\hline
6 & \vcltopframe{figures/content/appendix_d/episodes/cliff_mimovl7/frame_005.png} & \raggedright\ttfamily The character is getting closer to the right edge. Moving right again is still the way to go. The target is near the right edge, so keep moving right. Reasoning: The character is on the safe green platform and moving right is necessary to get closer to the target on the far right while avoiding the cliff. & \texttt{Right} & \vcltopframe{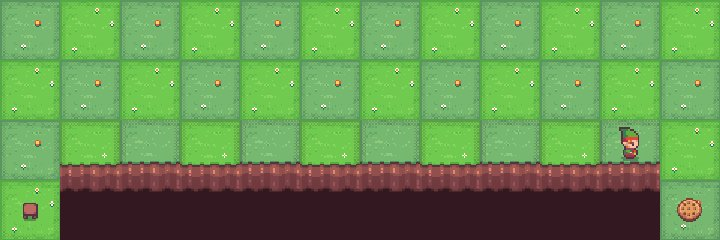} \\
\arrayrulecolor{black!12}\hline
7 & \vcltopframe{figures/content/appendix_d/episodes/cliff_mimovl7/frame_006.png} & \raggedright\ttfamily The character is very close to the target now. Moving right will get them even closer. The platform is still green, so right is safe. Reasoning: The character is on the safe green platform, and moving right is the logical next step to reach the target on the far right without falling. & \texttt{Right} & \vcltopframe{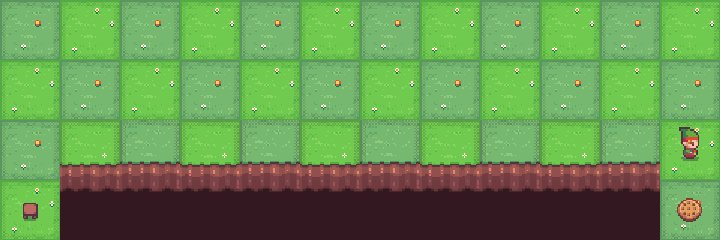} \\
\arrayrulecolor{black!12}\hline
8 & \vcltopframe{figures/content/appendix_d/episodes/cliff_mimovl7/frame_007.png} & \raggedright\ttfamily The character is now just a few squares from the target. Moving right one more time will get them closer. The platform is still green, so right is the best move. Reasoning: The character is on the safe green platform and moving right is the optimal action to reach the target on the far right while avoiding the cliff. & \texttt{Right} & \vcltopframe{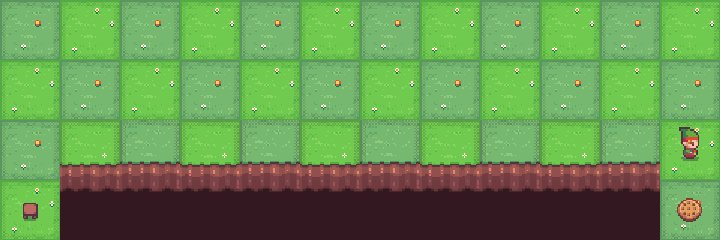} \\
\arrayrulecolor{black!12}\hline
9 & \vcltopframe{figures/content/appendix_d/episodes/cliff_mimovl7/frame_008.png} & \raggedright\ttfamily The character is almost at the target. Wait, in the example video, when they got close, they might have moved right again. But let's check: the target is a brown circle. The character is one square left of the target. So moving right would reach the target? Wait, no, the example video's step 10 was down, but maybe in that example it was a different path. Wait, no, the current task is to not fall. Wait, the target is on the right edge. Wait, the character is on the rightmost green square. Wait, no, the image shows the character is at the right edge of the green platform. Wait, no, the target is a brown circle. Wait, maybe the next step is right to get to the target. Wait, no, the character is next to the target? Wait, no, let's look again. The image: the character is on the rightmost green square, and the target is a brown circle to the right of that? No, the target is a brown circle on the right edge. Wait, no, the user's previous action was right, so the character is moving right. Wait, maybe the target is the brown circle, so when the character is next to it, maybe right is still the way. Wait, no, the example video's step 10 was down, but that was a different path. Wait, no, the current state: the character is on the green platform, target is on the right. So moving right is still correct. Reasoning: The character is on the safe green platform, and moving right is the logical next step to reach the target (brown circle) on the far right while staying above the cliff. & \texttt{Right} & \vcltopframe{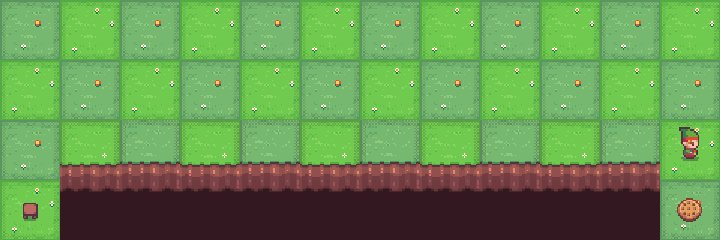} \\
\arrayrulecolor{black!12}\hline
10 & \vcltopframe{figures/content/appendix_d/episodes/cliff_mimovl7/frame_009.png} & \raggedright\ttfamily The character is now at the rightmost green square. The target is the brown circle. Wait, in the example video, step 10 was down, but maybe that's not the case here. Wait, no, the target is probably the brown circle. Wait, the user's goal is to reach the target. Wait, the character is on the green platform. Wait, maybe the target is the brown circle, so when the character is next to it, but in the image, the character is at the right edge. Wait, no, let's think again. The cliff is below, so if the character moves right, they might fall? No, the green squares are the safe platform. Wait, the target is on the right edge. Wait, maybe the action is Right again? No, wait, the example video's step 10 was down, but that was a different scenario. Wait, no, the current state: the character is on the green platform. Let's check the example: in the first video, they moved right until the end, then maybe down? Wait, no, the example's step 10 was down. Wait, maybe when you reach the end of the green platform, you have to move down? No, the cliff is below. Wait, no, the target is the brown circle. Wait, maybe the target is the brown circle, so the character needs to move right to reach it. Wait, the image shows the character is one square left of the target. Wait, no, the target is a brown circle on the right edge. So moving right would make the character reach the target. Wait, but the example video's step 10 was down. Hmm. Wait, no, the user's current state: the character is on the green platform. Let's decide: moving right is still the way. Reasoning: The character is on the safe green platform, and moving right is the next logical step to approach the target (brown circle) on the far right while avoiding the cliff below. & \texttt{Right} & \vcltopframe{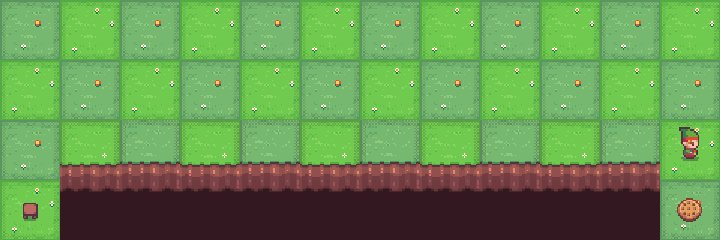} \\
\arrayrulecolor{black!12}\hline
11 & \vcltopframe{figures/content/appendix_d/episodes/cliff_mimovl7/frame_010.png} & \raggedright\ttfamily Wait, the example video's step 10 was Down. Let's think: the character is at the right edge of the green platform. If we move down, does that get them to the target? Wait, the target is a brown circle. Wait, maybe the target is on the lower level? No, the example video's step 10 was Down and led to Victory. Wait, in the example, the character moved down at step 10. So maybe here, moving down is the way. Wait, the current state: the character is on the green platform. If we move down, does that land them on the target? Wait, the target is a brown circle. Wait, maybe the target is the brown circle, and moving down is the correct action. Wait, let's check the example: in the example, step 10 was Action: Down and then Victory. So maybe when you reach the right edge, you move down. Wait, the user's step 10: the character is at the right edge. So move down. Reasoning: In the example gameplay, moving down at step 10 led to victory. The current state shows the character at the right edge of the green platform; moving down is the logical next step to reach the target (consistent with the example's successful strategy). & \texttt{Down} & \vcltopframe{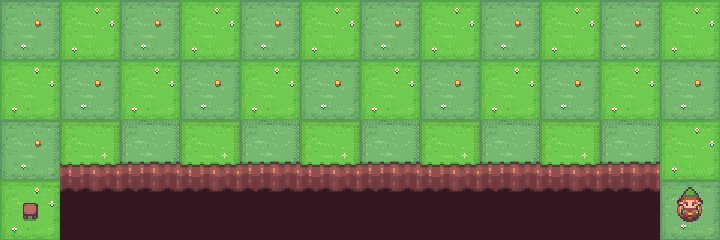} \\
\end{longtable}
\arrayrulecolor{black}
\endgroup

\begingroup
\scriptsize
\setlength{\tabcolsep}{2pt}
\renewcommand{\arraystretch}{1.05}
\arrayrulecolor{black!18}
\begin{longtable}{@{}c c p{8.0cm} c c@{}}
\caption{Complete same-start-state episode: Qwen3.6-27B on CliffWalking-v1 (4; victory; 8 steps; score 100).}
\label{tab:appendix-d-cliff-qwen3627}\\
\toprule
$t$ & Current state & Visible model rationale & Action & Next state \\
\midrule
\endfirsthead
\multicolumn{5}{c}{\tablename\ \thetable\ (continued)}\\
\toprule
$t$ & Current state & Visible model rationale & Action & Next state \\
\midrule
\endhead
\midrule
\multicolumn{5}{r}{Continued on next page}\\
\endfoot
\bottomrule
\endlastfoot
1 & \vcltopframe{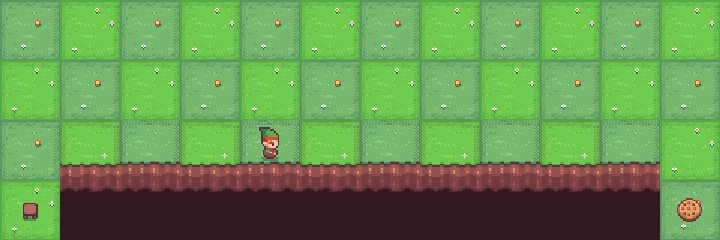} & \raggedright\ttfamily In the current initial state, the character is at the far left of the top row. The goal (the cookie) is at the bottom right corner. To reach it safely without falling off the cliff, the character must move along the top edge. Moving Right is the first step in this path. & \texttt{Right} & \vcltopframe{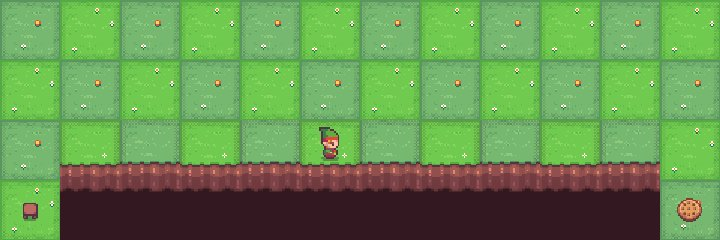} \\
\arrayrulecolor{black!12}\hline
2 & \vcltopframe{figures/content/appendix_d/episodes/cliff_qwen3627/frame_001.png} & \raggedright\ttfamily The character has moved one step to the right. The goal remains at the bottom right corner. To continue progressing toward the goal while staying on the safe upper path, the next logical move is to continue moving Right. & \texttt{Right} & \vcltopframe{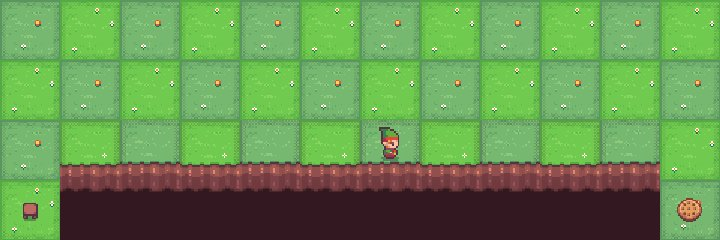} \\
\arrayrulecolor{black!12}\hline
3 & \vcltopframe{figures/content/appendix_d/episodes/cliff_qwen3627/frame_002.png} & \raggedright\ttfamily The character is still on the top row, moving towards the right side of the map. To reach the goal at the bottom right, the character needs to continue traversing the top edge safely. Moving Right is the correct next step. & \texttt{Right} & \vcltopframe{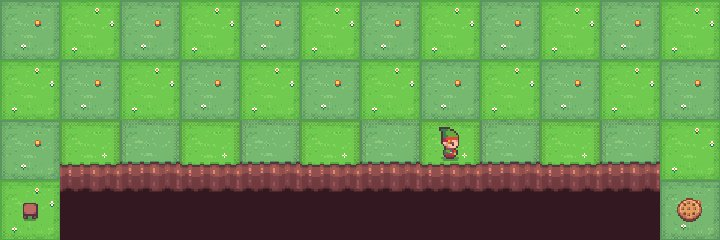} \\
\arrayrulecolor{black!12}\hline
4 & \vcltopframe{figures/content/appendix_d/episodes/cliff_qwen3627/frame_003.png} & \raggedright\ttfamily The character continues to move along the safe top row towards the right. The goal is still at the bottom right corner. To make progress, the character must keep moving Right until it reaches the far right edge, where it can then move down. & \texttt{Right} & \vcltopframe{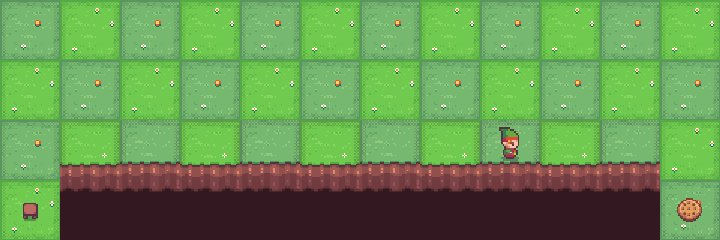} \\
\arrayrulecolor{black!12}\hline
5 & \vcltopframe{figures/content/appendix_d/episodes/cliff_qwen3627/frame_004.png} & \raggedright\ttfamily The character is progressing along the top row towards the right edge. The goal is at the bottom right. Continuing to move Right is necessary to reach the corner where the character can safely descend to the goal. & \texttt{Right} & \vcltopframe{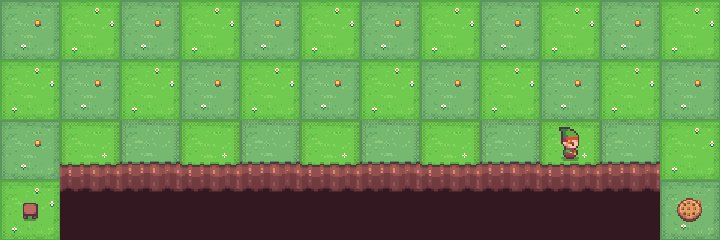} \\
\arrayrulecolor{black!12}\hline
6 & \vcltopframe{figures/content/appendix_d/episodes/cliff_qwen3627/frame_005.png} & \raggedright\ttfamily The character is now very close to the right edge of the top row. To reach the goal at the bottom right, the character needs to move one more step Right to get to the corner, and then it will be able to move Down safely. & \texttt{Right} & \vcltopframe{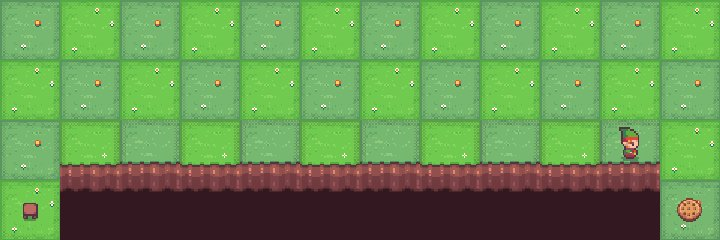} \\
\arrayrulecolor{black!12}\hline
7 & \vcltopframe{figures/content/appendix_d/episodes/cliff_qwen3627/frame_006.png} & \raggedright\ttfamily The character has reached the top-right corner of the safe path. The goal is directly below in the bottom-right corner. To align with the goal and prepare for the descent, the character must move one final step Right to be directly above the vertical column leading to the cookie. & \texttt{Right} & \vcltopframe{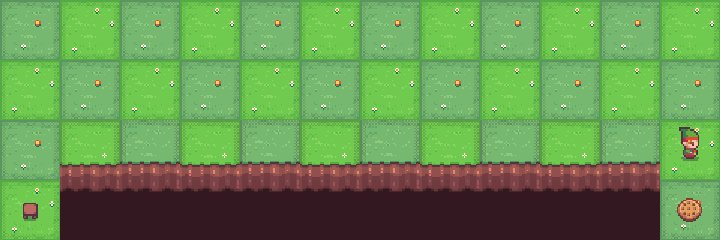} \\
\arrayrulecolor{black!12}\hline
8 & \vcltopframe{figures/content/appendix_d/episodes/cliff_qwen3627/frame_007.png} & \raggedright\ttfamily The character is now at the top-right corner, directly above the goal. The next logical step is to move Down towards the cookie. Moving Down will bring the character closer to the goal while staying on the safe path. & \texttt{Down} & \vcltopframe{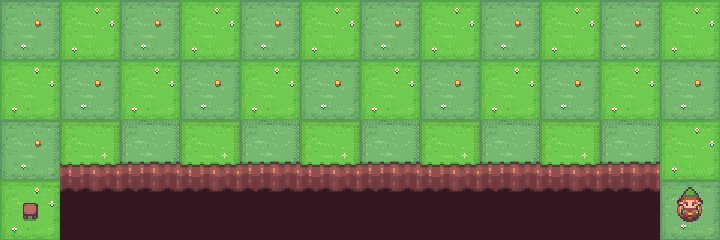} \\
\end{longtable}
\arrayrulecolor{black}
\endgroup

\begingroup
\scriptsize
\setlength{\tabcolsep}{2pt}
\renewcommand{\arraystretch}{1.05}
\arrayrulecolor{black!18}
\begin{longtable}{@{}c c p{8.0cm} c c@{}}
\caption{Complete same-start-state episode: GLM-4.5V on CliffWalking-v1 (4; gameover; 7 steps; score 77.14).}
\label{tab:appendix-d-cliff-glm45v}\\
\toprule
$t$ & Current state & Visible model rationale & Action & Next state \\
\midrule
\endfirsthead
\multicolumn{5}{c}{\tablename\ \thetable\ (continued)}\\
\toprule
$t$ & Current state & Visible model rationale & Action & Next state \\
\midrule
\endhead
\midrule
\multicolumn{5}{r}{Continued on next page}\\
\endfoot
\bottomrule
\endlastfoot
1 & \vcltopframe{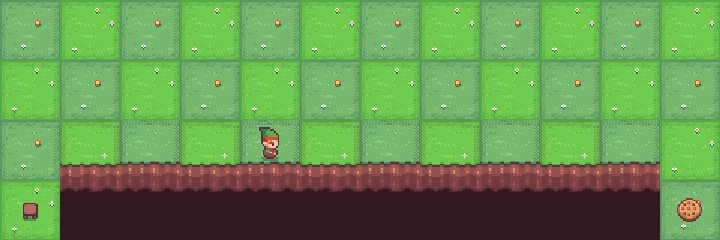} & \raggedright\ttfamily Got it, let's figure out the best action here. First, I need to understand the game's layout. The current state shows the player's position. Looking at the example gameplay, the goal is to reach the cookie on the right without falling off the cliff. The cliff is the brown area below, so we need to avoid that. In the initial state, the player is somewhere in the middle-left area. The example showed moving right to get towards the goal. Wait, but let's check the position. The player is on a green tile, and the cliff is below. So we need to move towards the right to reach the cookie. But maybe first, check if moving right is safe. Since the cliff is below, moving right on the green tiles is safe. The example gameplay had the player moving right multiple times to get closer. So the best action here is probably Right to start moving towards the goal. The goal is to reach the cookie on the right while avoiding the cliff. In the initial state, moving right progresses toward the target without immediate risk, as the cliff is below and the current tile is safe. Following the example gameplay's approach of moving right to advance toward the goal is logical. & \texttt{Right} & \vcltopframe{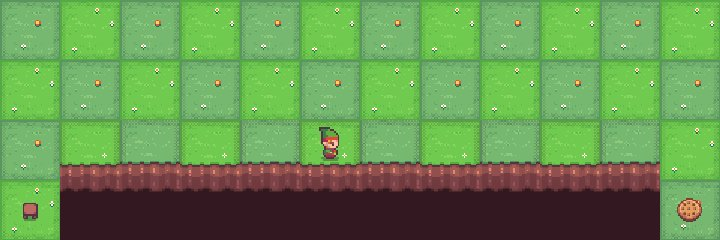} \\
\arrayrulecolor{black!12}\hline
2 & \vcltopframe{figures/content/appendix_d/episodes/cliff_glm45v/frame_001.png} & \raggedright\ttfamily Got it, let's see. The current state is after moving Right once. The character is now in the middle of the grid, still on the grass. The goal is to get to the cookie on the right. So the next step should be to continue moving Right to progress toward the cookie. That makes sense because moving right will get closer to the target without falling into the cliff (since the cliff is below, and we're on the grass tiles above). So the action should be Right again. The character is currently on a safe grass tile, and the goal (cookie) is to the right. Continuing to move Right progresses toward the target without immediate risk, as the cliff is below and the current position is safe. This aligns with the strategy of advancing toward the goal while avoiding hazards. & \texttt{Right} & \vcltopframe{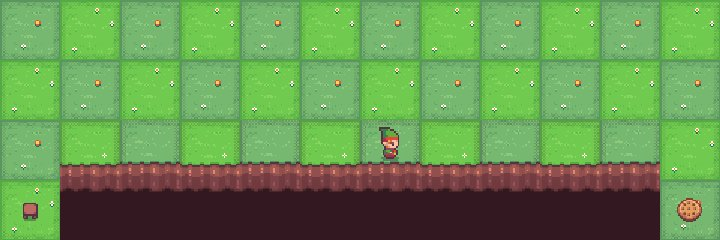} \\
\arrayrulecolor{black!12}\hline
3 & \vcltopframe{figures/content/appendix_d/episodes/cliff_glm45v/frame_002.png} & \raggedright\ttfamily Got it, let's see. The current state shows the character is on a grass tile, and the goal is the cookie on the right. The previous action was Right, so we need to keep moving towards the cookie. The cliff is below, so as long as we don't go down, we're safe. Moving Right again will get us closer to the cookie. So the next action should be Right. The character is on a safe grass tile, and the cookie (goal) is to the right. Continuing to move Right progresses toward the target without immediate risk, as the cliff is below and the current position is safe. This maintains the strategy of advancing toward the goal while avoiding hazards. & \texttt{Right} & \vcltopframe{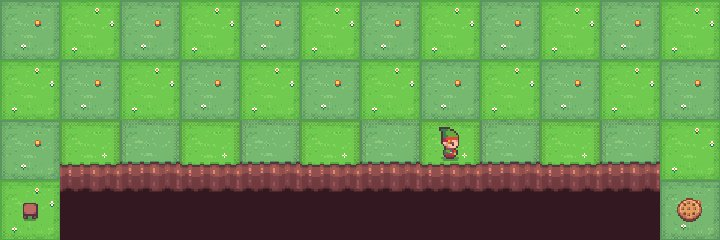} \\
\arrayrulecolor{black!12}\hline
4 & \vcltopframe{figures/content/appendix_d/episodes/cliff_glm45v/frame_003.png} & \raggedright\ttfamily Got it, let's see. The current state shows the character is still moving right. The goal is to get to the cookie on the right. Since the previous actions were right, and the character is progressing toward the cookie, the next logical step is to keep moving right. The cliff is below, so as long as we stay on the grass tiles, moving right is safe. So the action should be Right. The character is on a safe grass tile, and the cookie (goal) is to the right. Continuing to move Right progresses toward the target without immediate risk, as the cliff is below and the current position is safe. This maintains the strategy of advancing toward the goal while avoiding hazards. & \texttt{Right} & \vcltopframe{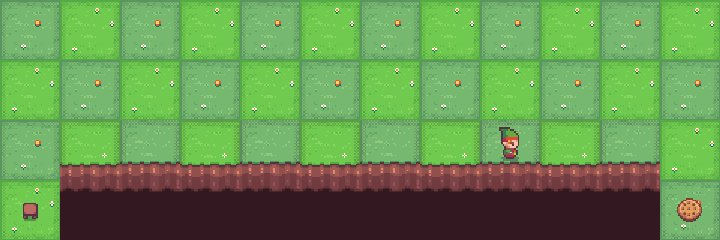} \\
\arrayrulecolor{black!12}\hline
5 & \vcltopframe{figures/content/appendix_d/episodes/cliff_glm45v/frame_004.png} & \raggedright\ttfamily Got it, let's see. The current state shows the character is on a grass tile, and the goal (cookie) is to the right. The previous action was Right, so we need to keep moving towards the cookie. Since the cliff is below, moving Right is safe here. So the next action should be Right. The character is on a safe grass tile, and the cookie (goal) is to the right. Continuing to move Right progresses toward the target without immediate risk, as the cliff is below and the current position is safe. This maintains the strategy of advancing toward the goal while avoiding hazards. & \texttt{Right} & \vcltopframe{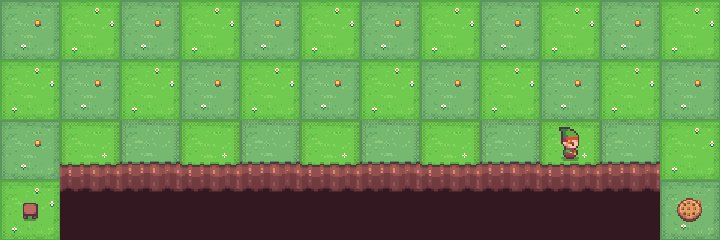} \\
\arrayrulecolor{black!12}\hline
6 & \vcltopframe{figures/content/appendix_d/episodes/cliff_glm45v/frame_005.png} & \raggedright\ttfamily Got it, let's see. The current state shows the character is on a grass tile, and the cookie is to the right. The previous action was Right, so we need to keep moving towards the cookie. The cliff is below, so as long as we stay on the grass, moving Right is safe. So the next action should be Right to get closer to the goal. The character is on a safe grass tile, and the cookie (goal) is to the right. Continuing to move Right progresses toward the target without immediate risk, as the cliff is below and the current position is safe. This maintains the strategy of advancing toward the goal while avoiding hazards. & \texttt{Right} & \vcltopframe{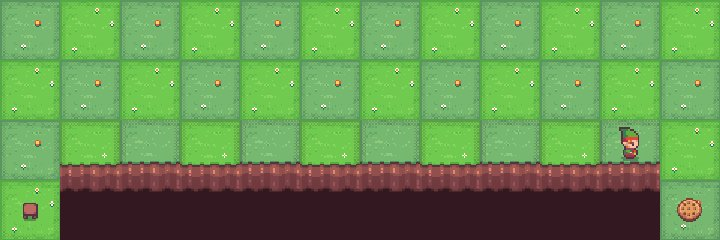} \\
\arrayrulecolor{black!12}\hline
7 & \vcltopframe{figures/content/appendix_d/episodes/cliff_glm45v/frame_006.png} & \raggedright\ttfamily Got it, let's see. The current state shows the character is on the rightmost grass tile, right next to the cookie. Wait, no, wait. Wait, the cookie is on the bottom right. Wait, the character is on the top right grass tile. So to get to the cookie, the character needs to go down, right? Because the cookie is below the cliff. Wait, no, wait. Wait, the cliff is the brown area. The cookie is on the bottom right, so the character is on the top right grass tile. So the next action should be Down to move down to the cliff? Wait, no, wait. Wait, in the example gameplay, when the character was on the right, they went Down to reach the cookie. Oh right, because the cookie is below the cliff. So the character needs to move Down from the top right grass tile to get to the cookie. So the next action is Down. The character is on the rightmost grass tile, adjacent to the cookie which is located below the cliff. To reach the cookie, the character must move Down from the current position. This action will position the character to collect the cookie and achieve victory. & \texttt{Down} & \vcltopframe{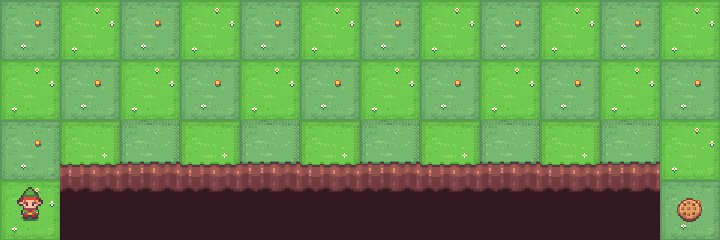} \\
\end{longtable}
\arrayrulecolor{black}
\endgroup

\begingroup
\scriptsize
\setlength{\tabcolsep}{2pt}
\renewcommand{\arraystretch}{1.05}
\arrayrulecolor{black!18}
\begin{longtable}{@{}c c p{8.0cm} c c@{}}
\caption{Complete same-start-state episode: Qwen3.5-VL-27B on CliffWalking-v1 (4; gameover; 7 steps; score 77.14).}
\label{tab:appendix-d-cliff-qwen35vl}\\
\toprule
$t$ & Current state & Visible model rationale & Action & Next state \\
\midrule
\endfirsthead
\multicolumn{5}{c}{\tablename\ \thetable\ (continued)}\\
\toprule
$t$ & Current state & Visible model rationale & Action & Next state \\
\midrule
\endhead
\midrule
\multicolumn{5}{r}{Continued on next page}\\
\endfoot
\bottomrule
\endlastfoot
1 & \vcltopframe{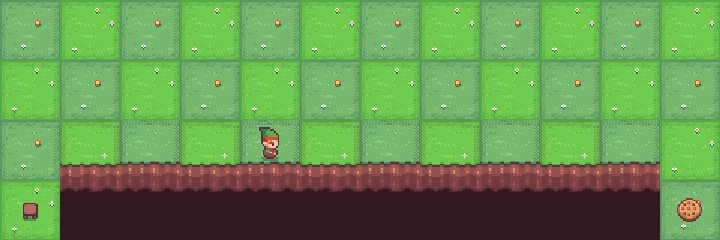} & \raggedright\ttfamily The character starts on the left side of the cliff, and the goal (cookie) is on the far right. Moving Right along the top safe path avoids the pit and progresses toward the goal, as demonstrated in the winning example. & \texttt{Right} & \vcltopframe{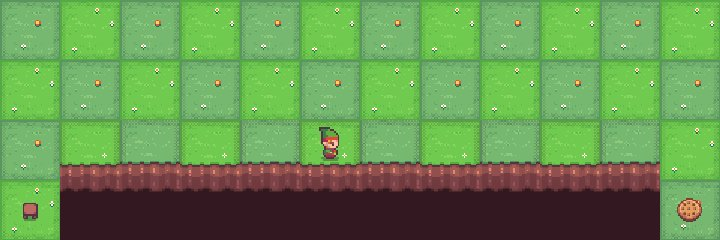} \\
\arrayrulecolor{black!12}\hline
2 & \vcltopframe{figures/content/appendix_d/episodes/cliff_qwen35vl/frame_001.png} & \raggedright\ttfamily The character has moved one step to the right and is still safely on the grass path. To reach the cookie on the far right, continuing to move Right is the correct path. Moving Down would cause the character to fall into the pit and lose. & \texttt{Right} & \vcltopframe{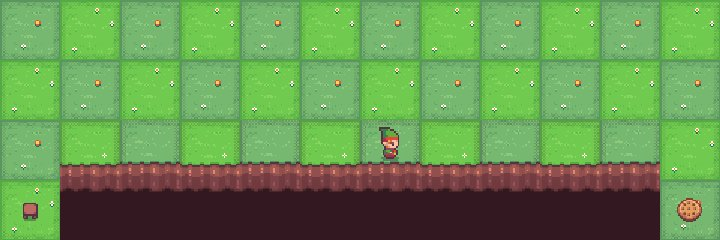} \\
\arrayrulecolor{black!12}\hline
3 & \vcltopframe{figures/content/appendix_d/episodes/cliff_qwen35vl/frame_002.png} & \raggedright\ttfamily The character is progressing safely along the top grassy ledge towards the goal on the right. Continuing to move Right maintains the safe path and gets closer to the cookie. Moving Down would result in falling into the pit. & \texttt{Right} & \vcltopframe{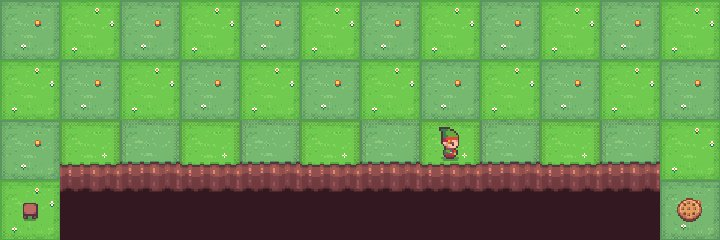} \\
\arrayrulecolor{black!12}\hline
4 & \vcltopframe{figures/content/appendix_d/episodes/cliff_qwen35vl/frame_003.png} & \raggedright\ttfamily The character continues to move along the safe upper path toward the cookie. There are no obstacles ahead, so moving Right is the optimal action to reach the goal. & \texttt{Right} & \vcltopframe{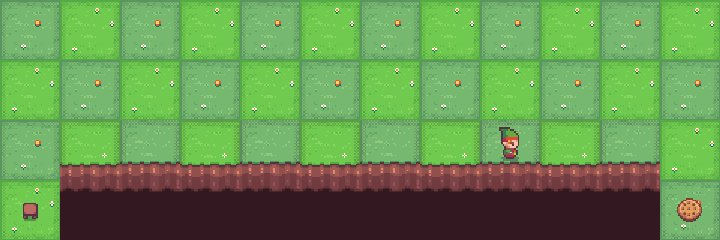} \\
\arrayrulecolor{black!12}\hline
5 & \vcltopframe{figures/content/appendix_d/episodes/cliff_qwen35vl/frame_004.png} & \raggedright\ttfamily The character is still on the safe grass path and needs to continue moving towards the right to reach the cookie. Moving Down would cause a fall into the pit, so Right remains the correct choice. & \texttt{Right} & \vcltopframe{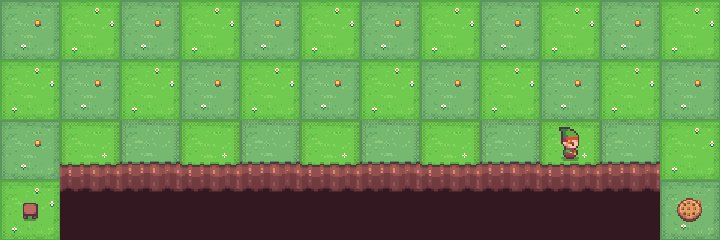} \\
\arrayrulecolor{black!12}\hline
6 & \vcltopframe{figures/content/appendix_d/episodes/cliff_qwen35vl/frame_005.png} & \raggedright\ttfamily The character is one step away from the vertical column where the cookie is located. Moving Right again will bring the character to the column directly above the cookie, from where they can safely move Down to collect it. & \texttt{Right} & \vcltopframe{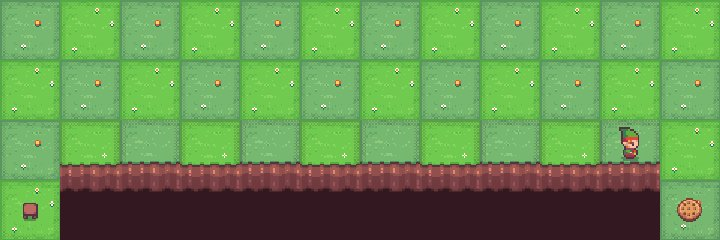} \\
\arrayrulecolor{black!12}\hline
7 & \vcltopframe{figures/content/appendix_d/episodes/cliff_qwen35vl/frame_006.png} & \raggedright\ttfamily The character has reached the column directly above the cookie. Moving Down is now safe and will allow the character to collect the cookie and win the game. & \texttt{Down} & \vcltopframe{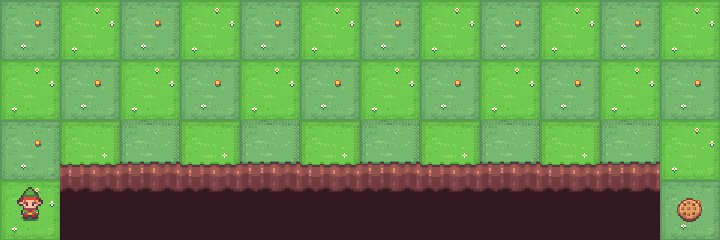} \\
\end{longtable}
\arrayrulecolor{black}
\endgroup

\begingroup
\scriptsize
\setlength{\tabcolsep}{2pt}
\renewcommand{\arraystretch}{1.05}
\arrayrulecolor{black!18}
\begin{longtable}{@{}c c p{8.0cm} c c@{}}
\caption{Complete same-start-state episode: Qwen3-Omni-30B on CliffWalking-v1 (4; victory; 9 steps; score 100).}
\label{tab:appendix-d-cliff-qwen3omni}\\
\toprule
$t$ & Current state & Visible model rationale & Action & Next state \\
\midrule
\endfirsthead
\multicolumn{5}{c}{\tablename\ \thetable\ (continued)}\\
\toprule
$t$ & Current state & Visible model rationale & Action & Next state \\
\midrule
\endhead
\midrule
\multicolumn{5}{r}{Continued on next page}\\
\endfoot
\bottomrule
\endlastfoot
1 & \vcltopframe{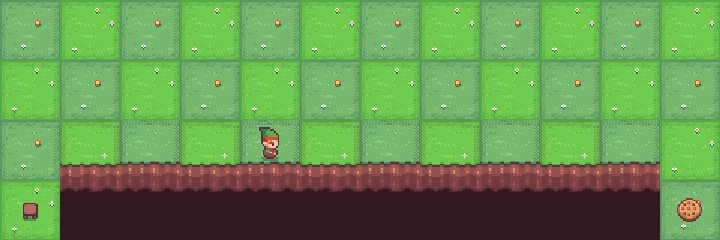} & \raggedright\emph{No visible rationale.} & \texttt{Right} & \vcltopframe{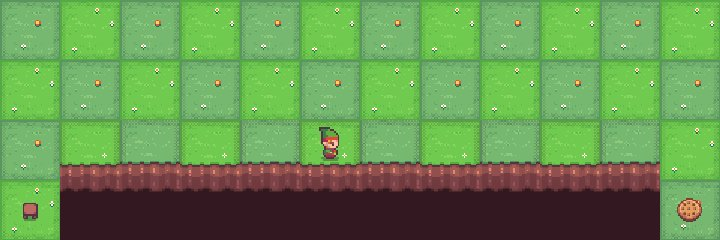} \\
\arrayrulecolor{black!12}\hline
2 & \vcltopframe{figures/content/appendix_d/episodes/cliff_qwen3omni/frame_001.png} & \raggedright\emph{No visible rationale.} & \texttt{Right} & \vcltopframe{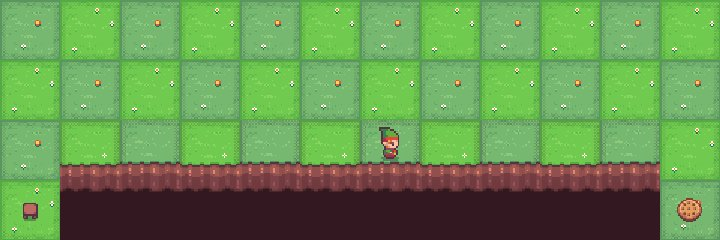} \\
\arrayrulecolor{black!12}\hline
3 & \vcltopframe{figures/content/appendix_d/episodes/cliff_qwen3omni/frame_002.png} & \raggedright\emph{No visible rationale.} & \texttt{Right} & \vcltopframe{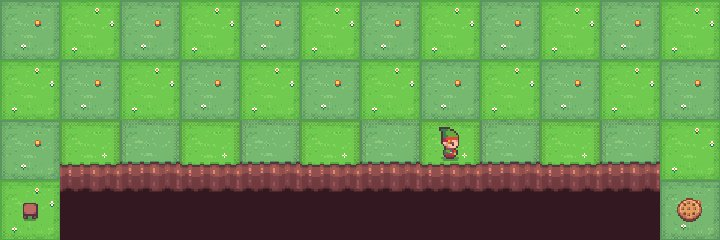} \\
\arrayrulecolor{black!12}\hline
4 & \vcltopframe{figures/content/appendix_d/episodes/cliff_qwen3omni/frame_003.png} & \raggedright\emph{No visible rationale.} & \texttt{Right} & \vcltopframe{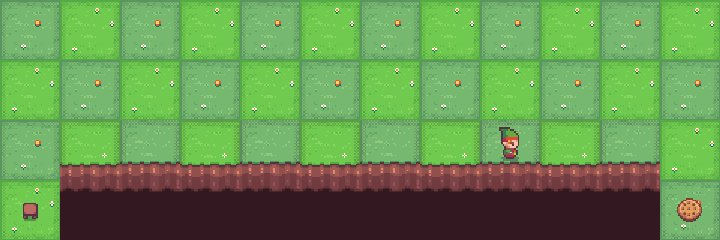} \\
\arrayrulecolor{black!12}\hline
5 & \vcltopframe{figures/content/appendix_d/episodes/cliff_qwen3omni/frame_004.png} & \raggedright\emph{No visible rationale.} & \texttt{Right} & \vcltopframe{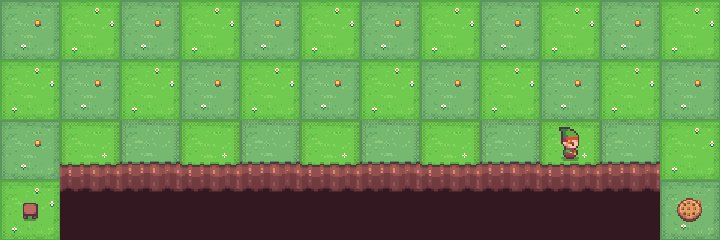} \\
\arrayrulecolor{black!12}\hline
6 & \vcltopframe{figures/content/appendix_d/episodes/cliff_qwen3omni/frame_005.png} & \raggedright\emph{No visible rationale.} & \texttt{Right} & \vcltopframe{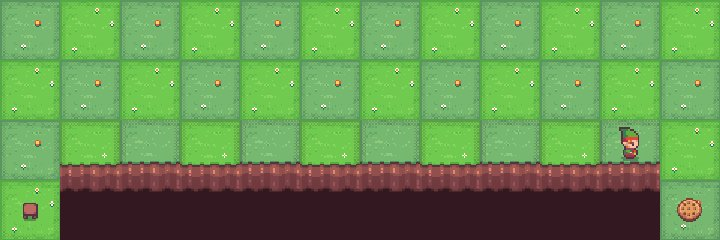} \\
\arrayrulecolor{black!12}\hline
7 & \vcltopframe{figures/content/appendix_d/episodes/cliff_qwen3omni/frame_006.png} & \raggedright\emph{No visible rationale.} & \texttt{Right} & \vcltopframe{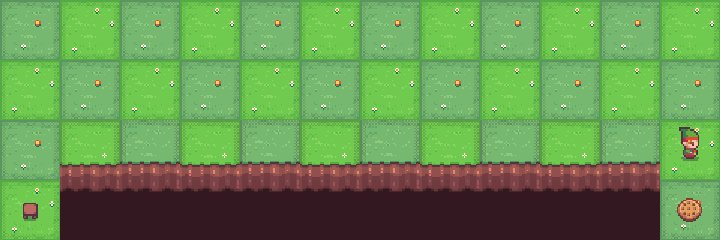} \\
\arrayrulecolor{black!12}\hline
8 & \vcltopframe{figures/content/appendix_d/episodes/cliff_qwen3omni/frame_007.png} & \raggedright\emph{No visible rationale.} & \texttt{Right} & \vcltopframe{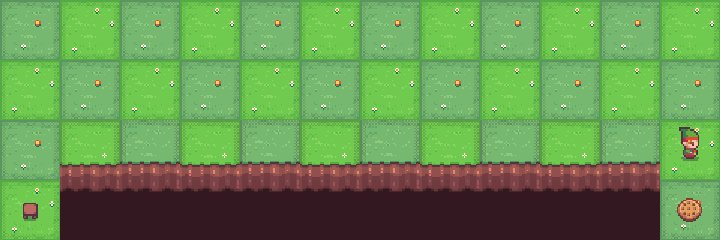} \\
\arrayrulecolor{black!12}\hline
9 & \vcltopframe{figures/content/appendix_d/episodes/cliff_qwen3omni/frame_008.png} & \raggedright\emph{No visible rationale.} & \texttt{Down} & \vcltopframe{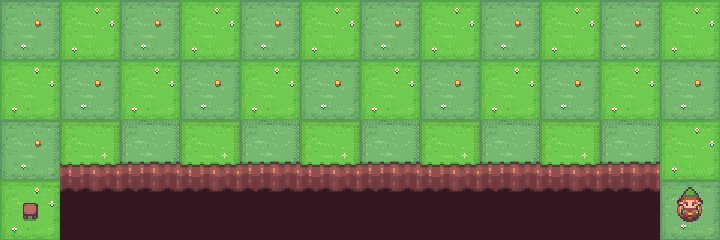} \\
\end{longtable}
\arrayrulecolor{black}
\endgroup

\begingroup
\scriptsize
\setlength{\tabcolsep}{2pt}
\renewcommand{\arraystretch}{1.05}
\arrayrulecolor{black!18}
\begin{longtable}{@{}c c p{8.0cm} c c@{}}
\caption{Complete same-start-state episode: Qwen3-VL-235B on CliffWalking-v1 (4; gameover; 6 steps; score 64.29).}
\label{tab:appendix-d-cliff-qwen3vl235}\\
\toprule
$t$ & Current state & Visible model rationale & Action & Next state \\
\midrule
\endfirsthead
\multicolumn{5}{c}{\tablename\ \thetable\ (continued)}\\
\toprule
$t$ & Current state & Visible model rationale & Action & Next state \\
\midrule
\endhead
\midrule
\multicolumn{5}{r}{Continued on next page}\\
\endfoot
\bottomrule
\endlastfoot
1 & \vcltopframe{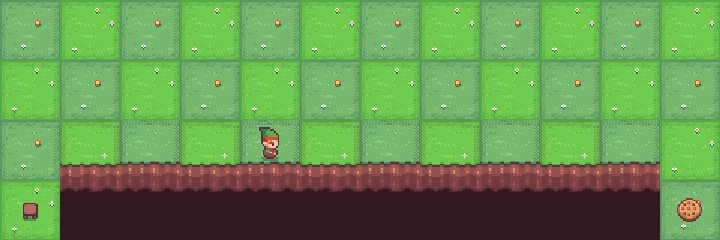} & \raggedright\ttfamily The current state shows the character positioned on the green grass above the cliff, with the goal (cookie) on the far right. Moving right aligns with the example gameplay where the character traversed rightward along the top row before descending to the cookie. Since the character is not yet at the rightmost column, proceeding right avoids falling off the cliff and progresses toward the target. & \texttt{Right} & \vcltopframe{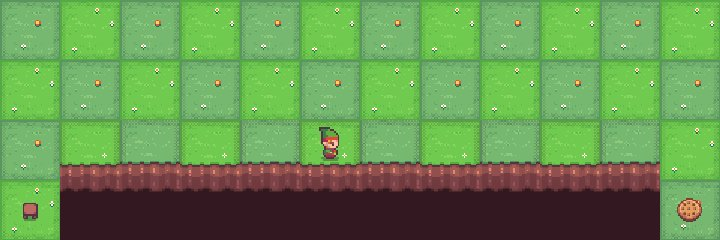} \\
\arrayrulecolor{black!12}\hline
2 & \vcltopframe{figures/content/appendix_d/episodes/cliff_qwen3vl235/frame_001.png} & \raggedright\emph{No visible rationale.} & \texttt{Right} & \vcltopframe{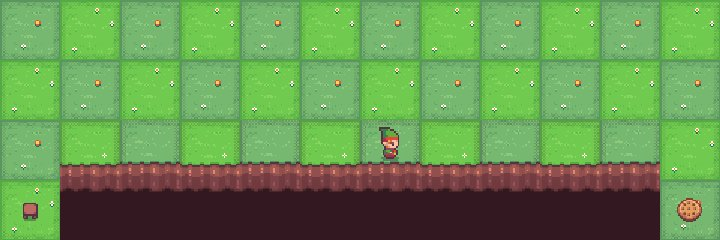} \\
\arrayrulecolor{black!12}\hline
3 & \vcltopframe{figures/content/appendix_d/episodes/cliff_qwen3vl235/frame_002.png} & \raggedright\emph{No visible rationale.} & \texttt{Right} & \vcltopframe{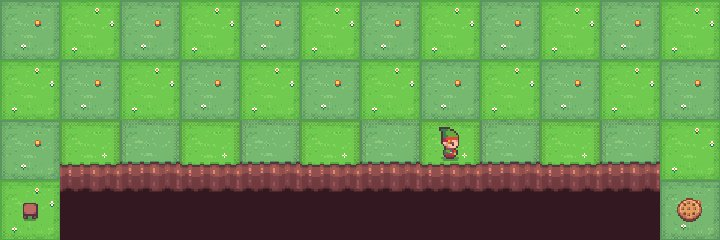} \\
\arrayrulecolor{black!12}\hline
4 & \vcltopframe{figures/content/appendix_d/episodes/cliff_qwen3vl235/frame_003.png} & \raggedright\emph{No visible rationale.} & \texttt{Right} & \vcltopframe{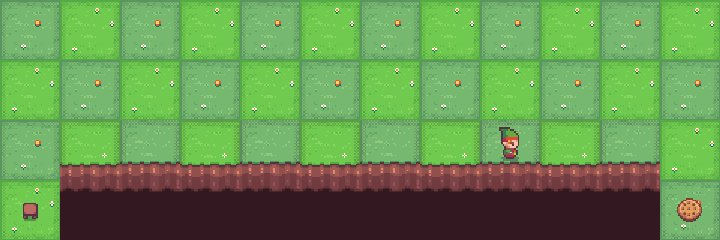} \\
\arrayrulecolor{black!12}\hline
5 & \vcltopframe{figures/content/appendix_d/episodes/cliff_qwen3vl235/frame_004.png} & \raggedright\emph{No visible rationale.} & \texttt{Right} & \vcltopframe{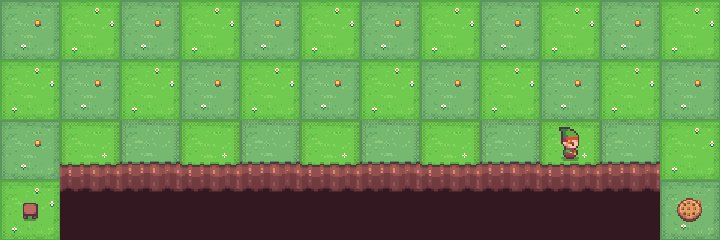} \\
\arrayrulecolor{black!12}\hline
6 & \vcltopframe{figures/content/appendix_d/episodes/cliff_qwen3vl235/frame_005.png} & \raggedright\emph{No visible rationale.} & \texttt{Down} & \vcltopframe{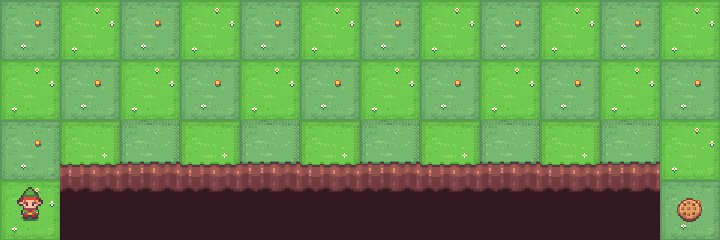} \\
\end{longtable}
\arrayrulecolor{black}
\endgroup
